# Supplementary material for: The $(2+\delta)$-dimensional theory of the electromechanics of lipid membranes: III. Constitutive models
Source: arXiv:2501.11612 ancillary file (2025-02-24)
Supplement: Supplementary file 1 [file thin_film_electromechanics_SI_part3.pdf]

# Supplemental Material

# The $(2+\delta)$-dimensional theory of the electromechanics of lipid membranes: III. Constitutive models

Yannick A. D. Omar [1,2,‡], Zachary G. Lipel [1,3], and Kranthi K. Mandadapu [1,4,§]

[1] Department of Chemical & Biomolecular Engineering, University of California, Berkeley, CA 94720, USA
[2] Department of Chemical Engineering, Massachusetts Institute of Technology, Cambridge, MA 02139, USA
[3] Department of Chemical & Biological Engineering, Princeton University, Princeton, NJ 08544, USA
[4] Chemical Sciences Division, Lawrence Berkeley National Laboratory, CA 94720, USA

## Contents

**1 Contravariant Basis Vector and Metric Tensor** **1**

**2 Derivation of Stresses and Moments** **3**
2.1 Elastic Response . . . 3
2.2 Viscous Response . . . 7
2.3 Mid-Surface Incompressibility . . . 12

**3 Equations of Motion** **14**
3.1 Elastic Response . . . 15
3.2 Viscous Response . . . 17
3.3 Reactive Stress Response . . . 17

**4 Traction Boundary Conditions** **18**

**5 Traction Boundary Conditions in Strict Surface Theories** **21**

**Supporting References** **23**

# 1 Contravariant Basis Vector and Metric Tensor

In Sec. 3 of the main text, we introduced the stress vectors $\boldsymbol{T}^i = \boldsymbol{\sigma}^T \boldsymbol{g}^i$ and expressed them as a series expansion in terms of Chebyshev polynomials, as derived in part 2 [1]. This series expansion contains inner products of the contravariant basis vectors with the Chebyshev polynomials, $\langle \boldsymbol{g}^\alpha, P_k(\Theta)\rangle$. Hence, evaluating the stress vectors $\boldsymbol{T}^i$ for a specific constitutive model requires an expression for the contravariant basis vectors in terms of Chebyshev polynomials. This was derived in detail in part 2 [1] and is summarized in the following along with an expansion for the contravariant metric tensor.

‡ yadomar@mit.edu
§ kranthi@berkeley.edu

We begin by recalling the expansion of the contravariant basis vectors in terms of the powers of the non-dimensional parametric direction $\Theta = 2/\delta\ \theta^3$ [1,2],

$$\boldsymbol{g}^\alpha = \sum_{m=0}^{\infty} \frac{1}{2^m} \boldsymbol{a}^\alpha \cdot \tilde{\boldsymbol{b}}^m \Theta^m \ , \tag{1}$$

where

$$\tilde{\boldsymbol{b}} = \delta \boldsymbol{b} \ , \tag{2}$$

is the non-dimensional curvature tensor, and $\boldsymbol{a}^\alpha$ are the contravariant basis vectors of the mid-surface defined in Sec. 2 of the main text. Given Eq. (1), we can find the contravariant metric tensor using the definition

$$g^{\alpha\beta} = \boldsymbol{g}^\alpha \cdot \boldsymbol{g}^\beta \ , \tag{3}$$

yielding

$$g^{\alpha\beta} = \sum_{i=0}^{\infty} \frac{i+1}{2^i} \boldsymbol{a}^\alpha \cdot \tilde{\boldsymbol{b}}^i \boldsymbol{a}^\beta \Theta^i \ . \tag{4}$$

To evaluate inner products involving Eqs. (1) and (4), we express them in terms of Chebyshev polynomials. To this end, we note that a monomial of non-negative order $m$ can be expressed in terms of Chebyshev polynomials as [3]

$$\Theta^m = \sum_{k=0}^{m} c_k \alpha_{mk} P_k(\Theta) \ , \tag{5}$$

where

$$c_k = \begin{cases} 1/2 \ , & \text{if } k = 0 \ , \\ 1 \ , & \text{otherwise} \ , \end{cases} \tag{6}$$

and

$$\alpha_{mk} = \begin{cases} 0 \ , & \text{if } m-k \text{ odd} \ , \\ 2^{1-m} \binom{m}{(m-k)/2} \ , & \text{if } m-k \text{ even} \ . \end{cases} \tag{7}$$

With this result, Eqs. (1) and (4) can be written, respectively, as

$$\boldsymbol{g}^\alpha = \sum_{m=0}^{\infty} \frac{1}{2^m} \boldsymbol{a}^\alpha \cdot \tilde{\boldsymbol{b}}^m \sum_{k=0}^{m} c_k \alpha_{mk} P_k(\Theta) \ , \tag{8}$$

and

$$g^{\alpha\beta} = \sum_{i=0}^{\infty} \frac{i+1}{2^i} \boldsymbol{a}^\alpha \cdot \tilde{\boldsymbol{b}}^i \boldsymbol{a}^\beta \sum_{k=0}^{i} c_k \alpha_{ik} P_k(\Theta) \ . \tag{9}$$

To evaluate the inner products of the contravariant basis vectors appearing in the stress vector expansions in Sec. 3 of the main text, we use the orthogonality relation $\langle P_k, P_l \rangle = \beta_k \delta_{kl}$ with $\beta_k$ defined in the main text and satisfying $\beta_k c_k = 1/2$. Thus, we obtain

$$\langle \boldsymbol{g}^\alpha, P_l(\Theta) \rangle = \frac{1}{2} \sum_{m=0}^{\infty} \frac{1}{2^m} \boldsymbol{a}^\alpha \cdot \tilde{\boldsymbol{b}}^m \alpha_{ml} \ . \tag{10}$$

## 2 Derivation of Stresses and Moments

In this section, we derive expressions for $N^{\alpha\beta}$, $M^{\alpha\beta}$, and $\boldsymbol{T}_2^\alpha$ for the elastic, viscous, and reactive stresses proposed in Secs. 4.1–4.3 of the main text. These allow us to specialize the constitutive model-independent equations of motion and boundary conditions to lipid membranes. To this end, we first expand the elastic, viscous, and reactive contributions to the stress vectors in terms of Chebyshev polynomials. Taking the appropriate inner products then yields the corresponding expressions for $N^{\alpha\beta}$, $M^{\alpha\beta}$, and $\boldsymbol{T}_2^\alpha$.

### 2.1 Elastic Response

We begin our derivations of the constitutive contributions to the equations of motion and boundary conditions by considering the elastic stress proposed in Sec. 4.1 of the main text. The associated in-plane stress vectors can be written as

$$\boldsymbol{T}_{\text{el}}^\alpha = \boldsymbol{\sigma}_{\text{el}}^T \boldsymbol{g}^\alpha = 2k_{\text{c}} \left(J-1\right) \boldsymbol{g}^\alpha \ , \tag{11}$$

where $J = \mathrm{d}v/\mathrm{d}V$ is the ratio of corresponding infinitesimal volume elements in the current and stress-free reference configurations. Using the assumption of Kirchhoff-Love kinematics, we can express the volume change $J$ using the change of surface area through the thickness [2, 4–6] to find

$$J = J_0 \, \frac{1 - \tilde{H}\Theta + \frac{1}{4}\tilde{K}\Theta^2}{1 - \tilde{C}\Theta + \frac{1}{4}\tilde{G}\Theta^2} \ , \tag{12}$$

where $J_0$ is the mid-surface stretch, $\tilde{H} = \delta H$ and $\tilde{K} = \delta^2 K$ are the non-dimensional mean and Gaussian curvatures of the current configuration, respectively, and $\tilde{C} = \delta C$ and $\tilde{G} = \delta^2 G$ are the non-dimensional mean and Gaussian curvatures of the stress-free reference configuration, respectively.

To express Eq. (12) in terms of Chebyshev polynomials, we first write the rational polynomial $\left(1 - \tilde{C}\Theta + \frac{1}{4}\tilde{G}\Theta^2\right)^{-1}$ using a series expansion. To this end, we first note that the assumption of small curvatures in the reference configuration discussed in Sec. 4.1 of the main text together with $\Theta \in (-1, 1)$ implies $|\tilde{C}\Theta| < 1$ and $|\tilde{G}\Theta^2| < 1$. Thus, we may Taylor-expand to obtain

$$\frac{1}{1 - \tilde{C}\Theta + \frac{1}{4}\tilde{G}\Theta^2} = \sum_{k=0}^{\infty} \sum_{n=0}^{\infty} \mu_{nk} \tilde{G}^k \tilde{C}^n \Theta^{2k+n} \ , \tag{13}$$

where

$$\mu_{nk} = \frac{(-1)^k}{4^k} \binom{n+k}{n} \ . \tag{14}$$

Substituting Eq. (13) into Eq. (12) then yields the series expansion

$$J = J_0 \sum_{k=0}^{\infty} \sum_{n=0}^{\infty} \mu_{nk} \tilde{G}^k \tilde{C}^n \left( \Theta^{2k+n} - \tilde{H}\Theta^{2k+n+1} + \frac{1}{4}\tilde{K}\Theta^{2(k+1)+n} \right) \ . \tag{15}$$

To evaluate $N^{\alpha\beta} = \delta \boldsymbol{T}_0^\alpha \cdot \boldsymbol{a}^\beta$ and $M^{\alpha\beta} = -\frac{\delta^2}{4}\boldsymbol{T}_1^\alpha \cdot \boldsymbol{a}^\beta$, we require the in-plane components of the stress vector in Eq. (11), i.e. $\boldsymbol{T}_{\mathrm{el}}^\alpha \cdot \boldsymbol{a}^\beta = 2k_{\mathrm{c}}\,(J-1)\,\boldsymbol{g}^\alpha \cdot \boldsymbol{a}^\beta$ (see Sec. 3 of the main text). Therefore, we use the series expansion of $\boldsymbol{g}^\alpha$ in Eq. (1) to find

$$\boldsymbol{g}^\alpha \cdot \boldsymbol{a}^\beta = \sum_{m=0}^{\infty} \frac{1}{2^m} \left[\tilde{\boldsymbol{b}}^m\right]^{\alpha\beta} \Theta^m \ , \tag{16}$$

which, in conjunction with Eq. (15), leads to

$$J\boldsymbol{g}^\alpha \cdot \boldsymbol{a}^\beta = J_0 \sum_{k=0}^{\infty}\sum_{n=0}^{\infty}\sum_{m=0}^{\infty} \frac{1}{2^m}\mu_{nk}\tilde{G}^k\tilde{C}^n \left[\tilde{\boldsymbol{b}}^m\right]^{\alpha\beta} \Big(\Theta^{2k+n+m} - \tilde{H}\Theta^{2k+n+1+m} + \frac{1}{4}\tilde{K}\Theta^{2(k+1)+n+m}\Big) \ . \tag{17}$$

To evaluate the inner product of Eq. (17) with the Chebyshev polynomials, we use Eq. (5) to obtain, for any $z \in \mathbb{N}_0^+$,

$$\langle \Theta^z, P_l(\Theta)\rangle = \frac{1}{2}\alpha_{zl} \ , \tag{18}$$

with $\alpha_{zl}$ given by Eq. (7).

Next, to find an expression for $N_{\mathrm{el}}^{\alpha\beta} = \langle \boldsymbol{T}_{\mathrm{el}}^\alpha \cdot \boldsymbol{a}^\beta, P_0(\Theta)\rangle$, we use Eq. (18) with $l = 0$ in Eq. (17) to find

$$2\left\langle \frac{J}{J_0}\boldsymbol{g}^\alpha \cdot \boldsymbol{a}^\beta, P_0(\Theta)\right\rangle = \sum_{k=0}^{\infty}\sum_{n=0}^{\infty}\sum_{m=0}^{\infty} \frac{1}{2^m}\mu_{nk}\tilde{G}^k\tilde{C}^n \left[\tilde{\boldsymbol{b}}^m\right]^{\alpha\beta} \times \Big(\alpha_{(2k+n+m)0} - \tilde{H}\alpha_{(2k+n+1+m)0} + \frac{1}{4}\tilde{K}\alpha_{(2(k+1)+n+m)0}\Big) \ . \tag{19}$$

The summations over $n$ and $k$ in Eq. (19) can be truncated using the assumption of small curvatures in the reference configuration, which yields

$$\begin{aligned} 2\left\langle \frac{J}{J_0}\boldsymbol{g}^\alpha \cdot \boldsymbol{a}^\beta, P_0(\Theta)\right\rangle = &\sum_{m=0}^{\infty} \frac{1}{2^m}\mu_{00} \left[\tilde{\boldsymbol{b}}^m\right]^{\alpha\beta} \Big(\alpha_{m0} - \tilde{H}\alpha_{(1+m)0} + \frac{1}{4}\tilde{K}\alpha_{(2+m)0}\Big) \\ &+ \sum_{m=0}^{\infty} \frac{1}{2^m}\mu_{10}\tilde{C} \left[\tilde{\boldsymbol{b}}^m\right]^{\alpha\beta} \Big(\alpha_{(1+m)0} - \tilde{H}\alpha_{(2+m)0} + \frac{1}{4}\tilde{K}\alpha_{(3+m)0}\Big) \\ &+ \sum_{m=0}^{\infty} \frac{1}{2^m}\mu_{20}\tilde{C}^2 \left[\tilde{\boldsymbol{b}}^m\right]^{\alpha\beta} \Big(\alpha_{(2+m)0} - \tilde{H}\alpha_{(3+m)0} + \frac{1}{4}\tilde{K}\alpha_{(4+m)0}\Big) \\ &+ \sum_{m=0}^{\infty} \frac{1}{2^m}\mu_{01}\tilde{G} \left[\tilde{\boldsymbol{b}}^m\right]^{\alpha\beta} \Big(\alpha_{(2+m)0} - \tilde{H}\alpha_{(3+m)0} + \frac{1}{4}\tilde{K}\alpha_{(4+m)0}\Big) + \mathcal{O}\big(\tilde{\kappa}_0^3\big) \ , \end{aligned} \tag{20}$$

where $\tilde{\kappa}_0 = \max_\alpha |\delta\kappa_{0\alpha}|$ is the largest of the principal curvatures $\kappa_{0\alpha}$ of the reference configuration. Equation (20) can be further simplified by recalling a result derived in part 2 [1],

$$\boldsymbol{c} \cdot (\delta\boldsymbol{b})^k\,\boldsymbol{a}^\alpha = \mathcal{O}\Big(\tilde{\kappa}^k\Big)\,\boldsymbol{c}\cdot\boldsymbol{i}\boldsymbol{a}^\alpha \ , \tag{21}$$

where $\boldsymbol{c}$ is an arbitrary vector and $\tilde{\kappa} = \max_\alpha |\delta\kappa_\alpha|$ is the largest of the principal curvatures $\kappa_\alpha$ of the current configuration. Using Eq. (21) with $\boldsymbol{c} \equiv \boldsymbol{a}^\beta$ then permits truncation of the summations in Eq. (20) at $m = 1$, leading to[1]

$$\left\langle \frac{J}{J_0} \boldsymbol{g}^\alpha \cdot \boldsymbol{a}^\beta, P_0(\Theta) \right\rangle \approx a^{\alpha\beta} + \frac{1}{8} \left[\tilde{\boldsymbol{b}}^2\right]^{\alpha\beta} - \frac{1}{4}\left(\tilde{H} - \tilde{C}\right) \tilde{b}^{\alpha\beta} + \frac{1}{8}\left(\tilde{K} - \tilde{G}\right) a^{\alpha\beta} - \frac{1}{2}\tilde{C}\left(\tilde{H} - \tilde{C}\right) a^{\alpha\beta} \, . \tag{22}$$

To obtain an expression for $N_{\text{el}}^{\alpha\beta}$, we also require the inner product of Eq. (16) with the zeroth-order Chebyshev polynomial. Upon using Eq. (18), we obtain

$$\left\langle \boldsymbol{g}^\alpha \cdot \boldsymbol{a}^\beta, P_0(\Theta) \right\rangle = \frac{1}{2} \sum_{m=0}^{\infty} \frac{1}{2^m} \left[\tilde{\boldsymbol{b}}^m\right]^{\alpha\beta} \alpha_{m0} \tag{23}$$

$$\approx a^{\alpha\beta} + \frac{1}{8}\left[\tilde{\boldsymbol{b}}^2\right]^{\alpha\beta} \, , \tag{24}$$

where we again used Eq. (21) to truncate the series expansion. Taking the inner product of the stress vector in Eq. (11) with the zeroth-order Chebyshev polynomial and using Eqs. (22) and (24) finally yields the expression for $N_{\text{el}}^{\alpha\beta}$ in terms of the dimensional curvatures as

$$N_{\text{el}}^{\alpha\beta} \approx 2\bar{k}_{\text{c}} \left(J_0 - 1\right) a^{\alpha\beta} + \frac{k_{\text{b}}}{2}\left[\boldsymbol{b}^2\right]^{\alpha\beta}\left(J_0 - 1\right) + J_0 k_{\text{b}} \left( -\left(H - C\right)\left(2Ca^{\alpha\beta} + b^{\alpha\beta}\right) + \frac{1}{2}\left(K - G\right) a^{\alpha\beta} \right) \, , \tag{25}$$

$$\approx 2\bar{k}_{\text{c}} \left(J_0 - 1\right) a^{\alpha\beta} + J_0 k_{\text{b}} \left( -\left(H - C\right)\left(2Ca^{\alpha\beta} + b^{\alpha\beta}\right) + \frac{1}{2}\left(K - G\right) a^{\alpha\beta} \right) \, , \tag{26}$$

where we defined the effective bulk modulus and bending rigidity, respectively, as

$$\bar{k}_{\text{c}} = \delta k_{\text{c}} \, , \tag{27}$$

$$k_{\text{b}} = \frac{\delta^3 k_{\text{c}}}{2} \, , \tag{28}$$

and neglected the term highlighted in orange based on Eq. (21).

Next, we seek to find an expression for the elastic moments $M_{\text{el}}^{\alpha\beta} = -\frac{\delta^2}{2}\langle \boldsymbol{T}_{\text{el}}^\alpha \cdot \boldsymbol{a}^\beta, P_1 \rangle$. This requires evaluating the inner product of the elastic stress vector in Eq. (11) with the first-order Chebyshev polynomial. To this end, we start from Eq. (17) and use Eq. (18) to obtain

$$2\left\langle \frac{J}{J_0} \boldsymbol{g}^\alpha \cdot \boldsymbol{a}^\beta, P_1(\Theta) \right\rangle = \sum_{k=0}^{\infty}\sum_{n=0}^{\infty}\sum_{m=0}^{\infty} \frac{1}{2^m} \mu_{nk} \tilde{G}^k \tilde{C}^n \left[\tilde{\boldsymbol{b}}^m\right]^{\alpha\beta} \times \left( \alpha_{(2k+n+m)1} - \tilde{H}\alpha_{(2k+n+1+m)1} + \frac{1}{4}\tilde{K}\alpha_{(2(k+1)+n+m)1} \right) \, . \tag{29}$$

[1] Note that it may be tempting to neglect the terms in Eq. (22) that are small compared to the first term of the right-hand side, i.e. $a^{\alpha\beta}$. We shall not do so, as one must consider the nature of these higher-order terms with respect to the difference in the mid-plane stretch, $(J_0 - 1)\, a^{\alpha\beta}$, which could be arbitrarily small (cf. Eq. (26)).

Again using the assumption of small curvatures in the reference configuration, Eq. (29) simplifies to

$$
\begin{aligned}
2\left\langle \frac{J}{J_0}\boldsymbol{g}^\alpha \cdot \boldsymbol{a}^\beta, P_1(\Theta)\right\rangle &= \sum_{m=0}^{\infty} \frac{1}{2^m}\mu_{00}\left[\tilde{\boldsymbol{b}}^m\right]^{\alpha\beta}\left(\alpha_{m1} - \tilde{H}\alpha_{(1+m)1} + \frac{1}{4}\tilde{K}\alpha_{(2+m)1}\right) \\
&+ \sum_{m=0}^{\infty} \frac{1}{2^m}\mu_{10}\tilde{C}\left[\tilde{\boldsymbol{b}}^m\right]^{\alpha\beta}\left(\alpha_{(1+m)1} - \tilde{H}\alpha_{(2+m)1} + \frac{1}{4}\tilde{K}\alpha_{(3+m)1}\right) \\
&+ \sum_{m=0}^{\infty} \frac{1}{2^m}\mu_{20}\tilde{C}^2\left[\tilde{\boldsymbol{b}}^m\right]^{\alpha\beta}\left(\alpha_{(2+m)1} - \tilde{H}\alpha_{(3+m)1} + \frac{1}{4}\tilde{K}\alpha_{(4+m)1}\right) \\
&+ \sum_{m=0}^{\infty} \frac{1}{2^m}\mu_{01}\tilde{G}\left[\tilde{\boldsymbol{b}}^m\right]^{\alpha\beta}\left(\alpha_{(2+m)1} - \tilde{H}\alpha_{(3+m)1} + \frac{1}{4}\tilde{K}\alpha_{(4+m)1}\right) + \mathcal{O}\left(\tilde{\kappa}_0^3\right) ,
\end{aligned}
\tag{30}
$$

which, upon using Eq. (21), further reduces to

$$
\left\langle \frac{J}{J_0}\boldsymbol{g}^\alpha \cdot \boldsymbol{a}^\beta, P_1(\Theta)\right\rangle \approx \frac{1}{4}\tilde{b}^{\alpha\beta} - \frac{1}{2}\left(\tilde{H} - \tilde{C}\right)a^{\alpha\beta} . \tag{31}
$$

Similarly, we take the inner product of Eq. (16) and use Eq. (18) to find,

$$
\left\langle \boldsymbol{g}^\alpha \cdot \boldsymbol{a}^\beta, P_1(\Theta)\right\rangle = \frac{1}{2}\sum_{m=0}^{\infty}\frac{1}{2^m}\boldsymbol{a}^\alpha \cdot \tilde{\boldsymbol{b}}^m \boldsymbol{a}^\beta \alpha_{m1} \tag{32}
$$

$$
\approx \frac{1}{4}\tilde{b}^{\alpha\beta} , \tag{33}
$$

with the second equality following from Eq. (21). Combing Eqs. (31) and (33) then yields the elastic contribution to the moments as

$$
M_{\mathrm{el}}^{\alpha\beta} \approx -\frac{k_{\mathrm{b}}}{2}\left(J_0 - 1\right)b^{\alpha\beta} + J_0 k_{\mathrm{b}}\left(H - C\right)a^{\alpha\beta} . \tag{34}
$$

To evaluate the constitutive parts of the traction boundary conditions (see Sec. 3 of the main text), we also require an expression for the elastic contribution to $\boldsymbol{T}_2^\alpha$, denoted by $\boldsymbol{T}_{2,\mathrm{el}}^\alpha$. To that end, we take the inner product of Eq. (17) with the second-order Chebyshev polynomial, resulting in

$$
\begin{aligned}
2\left\langle \frac{J}{J_0}\boldsymbol{g}^\alpha \cdot \boldsymbol{a}^\beta, P_2(\Theta)\right\rangle &= \sum_{k=0}^{\infty}\sum_{n=0}^{\infty}\sum_{m=0}^{\infty}\frac{1}{2^m}\mu_{nk}\tilde{G}^k\tilde{C}^n\left[\tilde{\boldsymbol{b}}^m\right]^{\alpha\beta} \times \\
&\left(\alpha_{(2k+n+m)2} - \tilde{H}\alpha_{(2k+n+1+m)2} + \frac{1}{4}\tilde{K}\alpha_{(2(k+1)+n+m)2}\right) .
\end{aligned}
\tag{35}
$$

As before, we use the assumption of small curvatures in the reference configuration to truncate the

summations over $n$ and $k$ to obtain

$$
\begin{aligned}
2\left\langle \frac{J}{J_0}\boldsymbol{g}^\alpha \cdot \boldsymbol{a}^\beta, P_2(\Theta)\right\rangle = &\sum_{m=0}^{\infty} \frac{1}{2^m}\mu_{00}\left[\tilde{\boldsymbol{b}}^m\right]^{\alpha\beta}\left(\alpha_{m2} - \tilde{H}\alpha_{(1+m)2} + \frac{1}{4}\tilde{K}\alpha_{(2+m)2}\right) \\
&+ \sum_{m=0}^{\infty} \frac{1}{2^m}\mu_{10}\tilde{C}\left[\tilde{\boldsymbol{b}}^m\right]^{\alpha\beta}\left(\alpha_{(1+m)2} - \tilde{H}\alpha_{(2+m)2} + \frac{1}{4}\tilde{K}\alpha_{(3+m)2}\right) \\
&+ \sum_{m=0}^{\infty} \frac{1}{2^m}\mu_{20}\tilde{C}^2\left[\tilde{\boldsymbol{b}}^m\right]^{\alpha\beta}\left(\alpha_{(2+m)2} - \tilde{H}\alpha_{(3+m)2} + \frac{1}{4}\tilde{K}\alpha_{(4+m)2}\right) \\
&+ \sum_{m=0}^{\infty} \frac{1}{2^m}\mu_{01}\tilde{G}\left[\tilde{\boldsymbol{b}}^m\right]^{\alpha\beta}\left(\alpha_{(2+m)2} - \tilde{H}\alpha_{(3+m)2} + \frac{1}{4}\tilde{K}\alpha_{(4+m)2}\right) + \mathcal{O}\left(\tilde{\kappa}_0^3\right) .
\end{aligned}
\tag{36}
$$

Using Eq. (21) further reduces Eq. (36) to

$$
\left\langle \frac{J}{J_0}\boldsymbol{g}^\alpha \cdot \boldsymbol{a}^\beta, P_2(\Theta)\right\rangle \approx \frac{1}{16}\left[\tilde{\boldsymbol{b}}^2\right]^{\alpha\beta} - \frac{1}{8}\left(\tilde{H} - \tilde{C}\right)\tilde{b}^{\alpha\beta} + \frac{1}{16}\left(\tilde{K} - \tilde{G}\right)a^{\alpha\beta} - \frac{1}{4}\tilde{C}\left(\tilde{H} - \tilde{C}\right)a^{\alpha\beta} . \tag{37}
$$

Finally, by taking the inner product of Eq. (16) with the second-order Chebyshev polynomial, we find

$$
\left\langle \boldsymbol{g}^\alpha \cdot \boldsymbol{a}^\beta, P_2(\Theta)\right\rangle = \frac{1}{2}\sum_{m=0}^{\infty}\frac{1}{2^m}\left[\tilde{\boldsymbol{b}}^m\right]^{\alpha\beta}\alpha_{m0} \tag{38}
$$

$$
\approx \frac{1}{16}\left[\tilde{\boldsymbol{b}}^2\right]^{\alpha\beta} . \tag{39}
$$

Combining Eqs. (37) and (39) then yields the expression for the elastic contribution to the second-order stress vector as

$$
\delta\boldsymbol{T}^\alpha_{2,\mathrm{el}} \cdot \boldsymbol{a}^\beta = 4k_\mathrm{c}\left(J_0\left\langle \frac{J}{J_0}\boldsymbol{g}^\alpha \cdot \boldsymbol{a}^\beta, P_2(\Theta)\right\rangle - \left\langle \boldsymbol{g}^\alpha \cdot \boldsymbol{a}^\beta, P_2(\Theta)\right\rangle\right) \tag{40}
$$

$$
\approx \frac{k_\mathrm{b}}{2}\left(J_0 - 1\right)b^\alpha_\gamma b^{\gamma\beta} + J_0 k_\mathrm{b}\left(-\left(H - C\right)\left(2Ca^{\alpha\beta} + b^{\alpha\beta}\right) + \frac{1}{2}\left(K - G\right)a^{\alpha\beta}\right) . \tag{41}
$$

## 2.2 Viscous Response

To evaluate the stresses and moments resulting from the viscous constitutive model

$$
\boldsymbol{\sigma}_\mathrm{visc} = 2\mu\,\boldsymbol{D} + \omega\mathrm{div}(\boldsymbol{v})\boldsymbol{1} , \tag{42}
$$

we first write the associated stress vectors $\boldsymbol{T}^\alpha_\mathrm{visc} = \boldsymbol{\sigma}^\mathrm{T}_\mathrm{visc}\boldsymbol{g}^\alpha$ as

$$
\boldsymbol{T}^\alpha_\mathrm{visc} = 2\mu\,\boldsymbol{i}\boldsymbol{D}\boldsymbol{g}^\alpha + \omega\mathrm{div}(\boldsymbol{v})\boldsymbol{g}^\alpha . \tag{43}
$$

Notice the projection of the viscous stresses onto the tangent plane using $\boldsymbol{i} = \boldsymbol{a}_\alpha \otimes \boldsymbol{a}^\alpha$ in Eq. (43). This is permissible since the stress components $\sigma_{i3} = \sigma_{3i}$ are determined by reactive stresses required to enforce Kirchhoff-Love kinematics, as discussed in Sec. 4 of the main text and in more detail in part 2 [1].

Expressing the shear viscosity term in Eq. (43) using Chebyshev polynomials requires an expansion of the symmetric part of velocity gradient $\boldsymbol{D} = \frac{1}{2}\left(\text{grad}(\boldsymbol{v}) + (\text{grad}(\boldsymbol{v}))^T\right)$. To this end, we write the velocity gradient and its symmetric part as

$$\text{grad}(\boldsymbol{v}) = \boldsymbol{v}_{,\alpha} \otimes \boldsymbol{g}^\alpha + \boldsymbol{v}_{,3} \otimes \boldsymbol{n} \ , \tag{44}$$

$$\boldsymbol{D} = \frac{1}{2}\left(\boldsymbol{v}_{,\alpha} \otimes \boldsymbol{g}^\alpha + \boldsymbol{g}^\alpha \otimes \boldsymbol{v}_{,\alpha} + \boldsymbol{v}_{,3} \otimes \boldsymbol{n} + \boldsymbol{n} \otimes \boldsymbol{v}_{,3}\right) \ . \tag{45}$$

From Eq. (45), we find that the term $\boldsymbol{iDg}^\alpha$ appearing in the stress vectors in Eq. (43) can be written as

$$\boldsymbol{iDg}^\alpha = \frac{1}{2}\left[\left(\boldsymbol{v}_{,\beta} \cdot \boldsymbol{a}^\gamma\right) g^{\alpha\beta} + \left(\boldsymbol{g}^\beta \cdot \boldsymbol{a}^\gamma\right)\left(\boldsymbol{v}_{,\beta} \cdot \boldsymbol{g}^\alpha\right)\right] \boldsymbol{a}_\gamma \ . \tag{46}$$

In the Supplementary Material of part 2 [1], we showed that the in-plane velocity gradient can be written as

$$\boldsymbol{v}_{,\alpha} = \left[w^\beta_{\cdot\,\alpha}\, \boldsymbol{a}_\beta + \left(v^\beta_0 b_{\beta\alpha} + v^3_{0,\alpha}\right) \boldsymbol{n}\right] P_0(\Theta) + \frac{\delta}{2}\left[v^\beta_{1:\alpha} \boldsymbol{a}_\beta + v^\beta_1 b_{\beta\alpha} \boldsymbol{n}\right] P_1(\Theta) \ , \tag{47}$$

with

$$w^\beta_{\cdot\,\alpha} = v^\beta_{0:\alpha} - v^3_0 b^\beta_\alpha \ . \tag{48}$$

By substituting Eqs. (9) and (47) into the first term of Eq. (46), we find

$$\begin{aligned}\left(\boldsymbol{v}_{,\beta} \cdot \boldsymbol{a}^\gamma\right) g^{\alpha\beta} = w^\gamma_{\cdot\,\beta} &\left(\sum_{m=0}^{\infty} \frac{m+1}{2^m} \boldsymbol{a}^\alpha \cdot \tilde{\boldsymbol{b}}^m \boldsymbol{a}^\beta \sum_{k=0}^{m} c_k \alpha_{mk} P_k(\Theta)\right) \\ &+ \frac{\delta}{2} v^\gamma_{1:\beta} \left(\sum_{m=0}^{\infty} \frac{m+1}{2^m} \boldsymbol{a}^\alpha \cdot \tilde{\boldsymbol{b}}^m \boldsymbol{a}^\beta \sum_{k=0}^{m+1} c_k \alpha_{(m+1)k} P_k(\Theta)\right) \ ,\end{aligned} \tag{49}$$

where we used $P_1(\Theta) = \Theta$ and Eq. (5). Similarly, we can write the second term of Eq. (46) from Eqs. (1) and (47) as

$$\begin{aligned}\left(\boldsymbol{g}^\beta \cdot \boldsymbol{a}^\gamma\right)\left(\boldsymbol{v}_{,\beta} \cdot \boldsymbol{g}^\alpha\right) = w^\mu_{\cdot\,\beta} &\left(\sum_{m=0}^{\infty} \frac{1}{2^m} \left[\tilde{\boldsymbol{b}}^m\right]^{\beta\gamma} \Theta^m\right)\left(\sum_{l=0}^{\infty} \frac{1}{2^l} \left[\tilde{\boldsymbol{b}}^l\right]^\alpha_\mu \Theta^l\right) \\ &+ \frac{\delta}{2} v^\mu_{1:\beta} \left(\sum_{m=0}^{\infty} \frac{1}{2^m} \left[\tilde{\boldsymbol{b}}^m\right]^{\beta\gamma} \Theta^m\right)\left(\sum_{l=0}^{\infty} \frac{1}{2^l} \left[\tilde{\boldsymbol{b}}^l\right]^\alpha_\mu \Theta^{l+1}\right)\end{aligned} \tag{50}$$

$$\begin{aligned}= w^\mu_{\cdot\,\beta} &\sum_{m=0}^{\infty} \sum_{l=0}^{m} \frac{1}{2^m} \left[\tilde{\boldsymbol{b}}^l\right]^{\beta\gamma} \left[\tilde{\boldsymbol{b}}^{m-l}\right]^\alpha_\mu \sum_{k=0}^{m} c_k \alpha_{mk} P_k(\Theta) \\ &+ \frac{\delta}{2} v^\mu_{1:\beta} \sum_{m=0}^{\infty} \sum_{l=0}^{m} \frac{1}{2^m} \left[\tilde{\boldsymbol{b}}^l\right]^{\beta\gamma} \left[\tilde{\boldsymbol{b}}^{m-l}\right]^\alpha_\mu \sum_{k=0}^{m+1} c_k \alpha_{(m+1)k} P_k(\Theta) \ .\end{aligned} \tag{51}$$

This concludes the series expansions for the individual terms in Eq. (46) associated with the shear viscosity term in Eq. (43).

Next, we seek to find a series expansion of the bulk viscosity term in Eq. (43). In the SM of part 2 [1], we showed that the divergence of the velocity can be written in terms of monomials $\Theta^m$ as

$$\mathrm{div}(\boldsymbol{v}) = \sum_{m=0}^{\infty} \frac{1}{2^m} \left[\tilde{\boldsymbol{b}}^m\right]^{\alpha}_{\beta} \left( w^{\beta}_{\cdot\alpha} \Theta^m + \frac{\delta}{2} v^{\beta}_{1:\alpha} \Theta^{m+1} \right) . \tag{52}$$

Multiplying Eq. (52) by the series expansion of the contravariant basis vector in Eq. (1) yields

$$\begin{aligned}
\mathrm{div}(\boldsymbol{v})\boldsymbol{g}^{\alpha} &= \sum_{m=0}^{\infty}\sum_{k=0}^{m} \frac{1}{2^m} \left[\tilde{\boldsymbol{b}}^{m-k}\right]^{\gamma}_{\beta} \left[\tilde{\boldsymbol{b}}^{k}\right]^{\alpha\mu} w^{\beta}_{\cdot\gamma}\, \boldsymbol{a}_{\mu}\, \Theta^m \\
&\qquad + \frac{\delta}{2} \sum_{m=0}^{\infty}\sum_{k=0}^{m} \frac{1}{2^m} \left[\tilde{\boldsymbol{b}}^{m-k}\right]^{\gamma}_{\beta} \left[\tilde{\boldsymbol{b}}^{k}\right]^{\alpha\mu} v^{\beta}_{1:\gamma}\, \boldsymbol{a}_{\mu}\, \Theta^{m+1} &(53) \\
&= \sum_{m=0}^{\infty}\sum_{k=0}^{m} \frac{1}{2^m} \left[\tilde{\boldsymbol{b}}^{m-k}\right]^{\gamma}_{\beta} \left[\tilde{\boldsymbol{b}}^{k}\right]^{\alpha\mu} w^{\beta}_{\cdot\gamma}\, \boldsymbol{a}_{\mu} \sum_{l=0}^{m} c_l \alpha_{ml} P_l(\Theta) \\
&\qquad + \frac{\delta}{2} \sum_{m=0}^{\infty}\sum_{k=0}^{m} \frac{1}{2^m} \left[\tilde{\boldsymbol{b}}^{m-k}\right]^{\gamma}_{\beta} \left[\tilde{\boldsymbol{b}}^{k}\right]^{\alpha\mu} v^{\beta}_{1:\gamma}\, \boldsymbol{a}_{\mu} \sum_{l=0}^{m+1} c_l \alpha_{(m+1)l} P_l(\Theta) \ , &(54)
\end{aligned}$$

where we again used Eq. (5).

We are now equipped to determine the viscous stress contribution $\pi^{\alpha\beta} = \delta\langle \boldsymbol{T}^{\alpha}_{\text{visc}} \cdot \boldsymbol{a}^{\beta}, P_0\rangle$. To that end, we first take the inner product of Eq. (46) with the zeroth-order Chebyshev polynomial and use Eqs. (18), (49) and (51) to obtain

$$\begin{aligned}
2\,\langle \boldsymbol{iDg}^{\alpha}, P_0(\Theta)\rangle \cdot \boldsymbol{a}^{\gamma} &= \frac{1}{2} w^{\gamma}_{\cdot\beta} \sum_{m=0}^{\infty} \frac{m+1}{2^m} \boldsymbol{a}^{\alpha} \cdot \tilde{\boldsymbol{b}}^m \boldsymbol{a}^{\beta} \alpha_{m0} \\
&\qquad + \frac{1}{2} w^{\mu}_{\cdot\beta} \sum_{m=0}^{\infty}\sum_{l=0}^{m} \frac{1}{2^m} \left[\tilde{\boldsymbol{b}}^{l}\right]^{\beta\gamma} \left[\tilde{\boldsymbol{b}}^{m-l}\right]^{\alpha}_{\mu} \alpha_{m0} \\
&\qquad + \frac{\delta}{4} v^{\gamma}_{1:\beta} \sum_{m=0}^{\infty} \frac{m+1}{2^m} \boldsymbol{a}^{\alpha} \cdot \tilde{\boldsymbol{b}}^m \boldsymbol{a}^{\beta} \alpha_{(m+1)0} \\
&\qquad + \frac{\delta}{4} v^{\mu}_{1:\beta} \sum_{m=0}^{\infty}\sum_{l=0}^{m} \frac{1}{2^m} \left[\tilde{\boldsymbol{b}}^{l}\right]^{\beta\gamma} \left[\tilde{\boldsymbol{b}}^{m-l}\right]^{\alpha}_{\mu} \alpha_{(m+1)0} &(55) \\
&= w^{\gamma}_{\cdot\beta} a^{\alpha\beta} + w^{\alpha}_{\cdot\beta} a^{\beta\gamma} + \frac{\delta^2}{8} \left( 2 v^{\gamma}_{1:\beta} b^{\alpha\beta} + v^{\mu}_{1:\beta} b^{\alpha}_{\mu} a^{\beta\gamma} + v^{\alpha}_{1:\beta} b^{\beta\gamma} \right) + \mathcal{O}\big(\tilde{\kappa}^2\big) \ , &(56)
\end{aligned}$$

where we used Eq. (21) to truncate the summations. Additionally, the terms highlighted in green in Eq. (56) can be shown to be small based on the existence of a characteristic velocity length scale $\ell_{\text{v}}$ (see Sec. 3 of the main text), $\tilde{\kappa}\, \left|\delta v^{\alpha}_1 / v^{\beta}_0\right| \ll 1$, and Eqs. (21) and (48), reducing Eq. (56) to

$$\langle \boldsymbol{iDg}^{\alpha}, P_0(\Theta)\rangle \cdot \boldsymbol{a}^{\gamma} \approx d^{\alpha\gamma}_0 - v^3_0 b^{\alpha\gamma} \ . \tag{57}$$

Here, $d^{\alpha\gamma}_0$ is the in-plane analog of the symmetric part of the velocity gradient, defined as

$$d^{\alpha\gamma}_0 = \frac{1}{2} \left( v^{\gamma}_{0:\beta} a^{\alpha\beta} + v^{\alpha}_{0:\beta} a^{\beta\gamma} \right) \ . \tag{58}$$

Similarly, taking the inner product of Eq. (54) yields

$$2\langle \operatorname{div}(\boldsymbol{v})\boldsymbol{g}^\alpha, P_0(\Theta)\rangle \cdot \boldsymbol{a}^\mu = \sum_{m=0}^{\infty}\sum_{k=0}^{m} \frac{1}{2^m}\left[\tilde{\boldsymbol{b}}^{m-k}\right]^{\gamma}_{\beta}\left[\tilde{\boldsymbol{b}}^{k}\right]^{\alpha\mu} w^{\beta}_{.\gamma}\,\alpha_{m0} + \frac{\delta}{2}\sum_{m=0}^{\infty}\sum_{k=0}^{m} \frac{1}{2^m}\left[\tilde{\boldsymbol{b}}^{m-k}\right]^{\gamma}_{\beta}\left[\tilde{\boldsymbol{b}}^{k}\right]^{\alpha\mu} v^{\beta}_{1:\gamma}\,\alpha_{(m+1)0}\ . \tag{59}$$

The summations can be truncated at the lowest non-vanishing order based on Eq. (21), simplifying Eq. (59) to

$$\langle \operatorname{div}(\boldsymbol{v})\boldsymbol{g}^\alpha, P_0(\Theta)\rangle \cdot \boldsymbol{a}^\mu = w^{\gamma}_{.\gamma}a^{\alpha\mu} + \frac{\delta^2}{4}\left(b^{\gamma}_{\beta}v^{\beta}_{1:\gamma}a^{\alpha\mu} + b^{\alpha\mu}v^{\beta}_{1:\beta}\right) + \mathcal{O}(\tilde{\kappa}^2)\ , \tag{60}$$

We can again invoke the characteristic length scale $\ell_{\mathrm{v}}$, $\tilde{\kappa}\left|\delta v^{\alpha}_{1}/v^{\beta}_{0}\right| \ll 1$, and Eqs. (21) and (48) to neglect the terms highlighted in green, yielding

$$\langle \operatorname{div}(\boldsymbol{v})\boldsymbol{g}^\alpha, P_0(\Theta)\rangle \cdot \boldsymbol{a}^\mu \approx \left(v^{\gamma}_{0:\gamma} - 2v^3_0 H\right)a^{\alpha\mu}\ . \tag{61}$$

Finally, by combining Eqs. (57) and (61), we obtain the viscous stress $\pi^{\alpha\beta}$ as

$$\pi^{\alpha\beta} \approx 2\zeta\left(d^{\alpha\beta}_0 - v^3_0 b^{\alpha\beta}\right) + \bar{\omega}\left(v^{\gamma}_{0:\gamma} - 2v^3_0 H\right)a^{\alpha\beta}\ , \tag{62}$$

where we defined the effective surface shear and bulk viscosities as

$$\zeta = \delta\mu\ , \tag{63}$$
$$\bar{\omega} = \delta\omega\ . \tag{64}$$

Even though it is commonly assumed that the viscous contributions to the moments are negligible, we now derive an expression for $M^{\alpha\beta}_{\mathrm{visc}} = -\frac{\delta^2}{2}\langle \boldsymbol{T}^{\alpha}_{\mathrm{visc}}\cdot\boldsymbol{a}^{\beta}, P_1\rangle$ for completeness. To this end, we take the inner product of Eq. (46) and use Eqs. (18), (49) and (51) to obtain

$$\begin{aligned}
4\,\langle \boldsymbol{iDg}^\alpha, P_1(\Theta)\rangle\cdot\boldsymbol{a}^\gamma = {} & w^{\gamma}_{.\beta}\left(\sum_{m=0}^{\infty}\frac{m+1}{2^m}\boldsymbol{a}^\alpha\cdot\tilde{\boldsymbol{b}}^m\boldsymbol{a}^\beta\alpha_{m1}\right) \\
& + w^{\mu}_{.\beta}\sum_{m=0}^{\infty}\sum_{l=0}^{m}\frac{1}{2^m}\left[\tilde{\boldsymbol{b}}^{l}\right]^{\beta\gamma}\left[\tilde{\boldsymbol{b}}^{m-l}\right]^{\alpha}_{\mu}\alpha_{m1} \\
& + \frac{\delta}{2}v^{\gamma}_{1:\beta}\sum_{m=0}^{\infty}\frac{m+1}{2^m}\boldsymbol{a}^\alpha\cdot\tilde{\boldsymbol{b}}^m\boldsymbol{a}^\beta\alpha_{(m+1)1} \\
& + \frac{\delta}{2}v^{\mu}_{1:\beta}\sum_{m=0}^{\infty}\sum_{l=0}^{m}\frac{1}{2^m}\left[\tilde{\boldsymbol{b}}^{l}\right]^{\beta\gamma}\left[\tilde{\boldsymbol{b}}^{m-l}\right]^{\alpha}_{\mu}\alpha_{(m+1)1}
\end{aligned} \tag{65}$$

$$= \delta w^{\gamma}_{.\beta}b^{\alpha\beta} + \frac{\delta}{2}w^{\mu}_{.\beta}\left(a^{\beta\gamma}b^{\alpha}_{\mu} + b^{\beta\gamma}\delta^{\alpha}_{\mu}\right) + \frac{\delta}{2}v^{\gamma}_{1:\beta}\,a^{\alpha\beta} + \frac{\delta}{2}v^{\alpha}_{1:\beta}\,a^{\beta\gamma} + \mathcal{O}(\tilde{\kappa}^2)\ , \tag{66}$$

where we also employed Eqs. (2) and (21), and the Kronecker delta $\delta^\alpha_\mu = a^\alpha_\mu$. Similarly, taking the inner product of Eq. (54) with the first-order Chebyshev polynomial produces

$$
\begin{aligned}
2\langle \mathrm{div}(\boldsymbol{v})\boldsymbol{g}^\alpha, P_1(\Theta)\rangle \cdot \boldsymbol{a}^\mu =& \sum_{m=0}^{\infty}\sum_{k=0}^{m} \frac{1}{2^m}\left[\tilde{\boldsymbol{b}}^{m-k}\right]^\gamma_\beta \left[\tilde{\boldsymbol{b}}^k\right]^{\alpha\mu} w^\beta_{.\gamma}\,\alpha_{m1} \\
&+ \frac{\delta}{2}\sum_{m=0}^{\infty}\sum_{k=0}^{m} \frac{1}{2^m}\left[\tilde{\boldsymbol{b}}^{m-k}\right]^\gamma_\beta \left[\tilde{\boldsymbol{b}}^k\right]^{\alpha\mu} v^\beta_{1:\gamma}\,\alpha_{(m+1)1} \qquad (67)\\
=& \frac{\delta}{4} v^\beta_{1:\beta} a^{\alpha\mu}\boldsymbol{a}_\mu + \frac{\delta}{4}\left(b^\gamma_\beta w^\beta_{.\gamma} a^{\alpha\mu} + w^\beta_{.\beta} b^{\alpha\mu}\right) + \mathcal{O}\left(\tilde{\kappa}^2\right)\ . \qquad (68)
\end{aligned}
$$

From Eqs. (66) and (68), we now find the viscous contributions to the moments as

$$
\begin{aligned}
M^{\alpha\beta}_{\text{visc}} \approx& -\frac{\delta^3\mu}{4}\left(w^\beta_{.\gamma} b^{\alpha\gamma} + \frac{1}{2} w^\mu_{.\gamma}\left(a^{\gamma\beta} b^\alpha_\mu + b^{\gamma\beta}\delta^\alpha_\mu\right) + v^\beta_{1:\gamma}\, a^{\alpha\gamma} + v^\alpha_{1:\gamma}\, a^{\gamma\beta}\right) \\
&- \frac{\omega\delta^3}{16}\left(v^\gamma_{1:\gamma} a^{\alpha\beta} + b^\gamma_\lambda w^\lambda_{.\gamma} a^{\alpha\beta} + w^\gamma_{.\gamma} b^{\alpha\beta}\right)\ . \qquad (69)
\end{aligned}
$$

Finally, we derive an expression for the viscous contribution to $\boldsymbol{T}^\alpha_2$, denoted by $\boldsymbol{T}^\alpha_{2,\text{visc}}$. We begin by taking the inner product of Eq. (46) with the second-order Chebyshev polynomial and use Eqs. (2) and (21) to obtain

$$
\begin{aligned}
2\left\langle \boldsymbol{iD}\boldsymbol{g}^\alpha, P_2(\Theta)\right\rangle =& w^\gamma_{.\beta}\sum_{m=0}^{\infty}\frac{m+1}{2^m}\boldsymbol{a}^\alpha\cdot\tilde{\boldsymbol{b}}^m\boldsymbol{a}^\beta\alpha_{m2}\boldsymbol{a}_\gamma \\
&+ w^\mu_{.\beta}\sum_{m=0}^{\infty}\sum_{l=0}^{m}\frac{1}{2^m}\left[\tilde{\boldsymbol{b}}^l\right]^{\beta\gamma}\left[\tilde{\boldsymbol{b}}^{m-l}\right]^\alpha_\mu \alpha_{m2}\,\boldsymbol{a}_\gamma \\
&+ \frac{\delta}{2} v^\gamma_{1:\beta}\sum_{m=0}^{\infty}\frac{m+1}{2^m}\boldsymbol{a}^\alpha\cdot\tilde{\boldsymbol{b}}^m\boldsymbol{a}^\beta\alpha_{(m+1)2}\,\boldsymbol{a}_\gamma + \\
&+ \frac{\delta}{2} v^\mu_{1:\beta}\sum_{m=0}^{\infty}\sum_{l=0}^{m}\frac{1}{2^m}\left[\tilde{\boldsymbol{b}}^l\right]^{\beta\gamma}\left[\tilde{\boldsymbol{b}}^{m-l}\right]^\alpha_\mu \alpha_{(m+1)2}\,\boldsymbol{a}_\gamma \qquad (70)\\
=& \frac{\delta^2}{8}\Big(3w^\gamma_{.\beta} b^{\alpha\lambda} b^\beta_\lambda + w^\mu_{.\beta}\left(b^{\beta\lambda} b^\gamma_\lambda \delta^\alpha_\mu + b^{\beta\gamma} b^\alpha_\mu + a^{\beta\gamma} b^{\alpha\lambda} b_{\lambda\mu}\right) \\
&+ \left(2v^\gamma_{1:\beta} b^{\alpha\beta} + v^\mu_{1:\beta}\left(a^{\beta\gamma} b^\alpha_\mu + b^{\beta\gamma}\delta^\alpha_\mu\right)\right)\Big)\boldsymbol{a}_\gamma + \mathcal{O}\left(\tilde{\kappa}^3\right)\ . \qquad (71)
\end{aligned}
$$

Analogously, the inner product of Eq. (54) with the second-order Chebyshev polynomials yields

$$
\begin{aligned}
2\langle \mathrm{div}(\boldsymbol{v})\boldsymbol{g}^\alpha, P_2(\Theta)\rangle =& \sum_{m=0}^{\infty}\sum_{k=0}^{m}\frac{1}{2^m}\left[\tilde{\boldsymbol{b}}^{m-k}\right]^\gamma_\beta\left[\tilde{\boldsymbol{b}}^k\right]^{\alpha\mu} w^\beta_{.\gamma}\alpha_{m2}\,\boldsymbol{a}_\mu \\
&+ \frac{\delta}{2}\sum_{m=0}^{\infty}\sum_{k=0}^{m}\frac{1}{2^m}\left[\tilde{\boldsymbol{b}}^{m-k}\right]^\gamma_\beta\left[\tilde{\boldsymbol{b}}^k\right]^{\alpha\mu} v^\beta_{1:\gamma}\,\alpha_{(m+1)2}\,\boldsymbol{a}_\mu \qquad (72)\\
=& \frac{\delta^2}{8}\Big(w^\beta_{.\gamma}\left(b^\gamma_\lambda b^\lambda_\beta a^{\alpha\mu} + b^\gamma_\beta b^{\alpha\mu} + \delta^\gamma_\beta b^\alpha_\lambda b^{\lambda\mu}\right) + \\
& v^\beta_{1:\gamma}\left(b^\gamma_\beta a^{\alpha\mu} + \delta^\gamma_\beta b^{\alpha\mu}\right)\Big)\boldsymbol{a}_\mu + \mathcal{O}\left(\tilde{\kappa}^3\right)\ , \qquad (73)
\end{aligned}
$$

such that we find

$$\boldsymbol{T}^{\alpha}_{2,\text{visc}} \approx \frac{\mu\delta^2}{4}\Big(3w^{\gamma}_{\ .\beta}b^{\alpha\lambda}b^{\beta}_{\lambda} + w^{\mu}_{\ .\beta}\Big(b^{\beta\lambda}b^{\gamma}_{\lambda}\delta^{\alpha}_{\mu} + b^{\beta\gamma}b^{\alpha}_{\mu} + a^{\beta\gamma}b^{\alpha\lambda}b_{\lambda\mu}\Big) + 2v^{\gamma}_{1:\beta}b^{\alpha\beta} + v^{\mu}_{1:\beta}\Big(a^{\beta\gamma}b^{\alpha}_{\mu} + b^{\beta\gamma}\delta^{\alpha}_{\mu}\Big)\Big)\,\boldsymbol{a}_{\gamma} + \frac{\omega\delta^2}{8}\Big(w^{\beta}_{\ .\gamma}\Big(b^{\gamma}_{\lambda}b^{\lambda}_{\beta}a^{\alpha\mu} + b^{\gamma}_{\beta}b^{\alpha\mu} + \delta^{\gamma}_{\beta}b^{\alpha}_{\lambda}b^{\lambda\mu}\Big) + v^{\beta}_{1:\gamma}\Big(b^{\gamma}_{\beta}a^{\alpha\mu} + \delta^{\gamma}_{\beta}b^{\alpha\mu}\Big)\Big)\,\boldsymbol{a}_{\mu}\ . \tag{74}$$

## 2.3 Mid-Surface Incompressibility

Since lipid membranes can only withstand a small mid-surface area stretch [7–9], they are commonly modeled as mid-surface area incompressible materials. To incorporate area incompressibility into the $(2+\delta)$-dimensional theory, we employ an approach similar to the enforcement of Kirchhoff-Love kinematics described in part 2 [1]. Specifically, we formulate the mid-surface incompressibility condition as a three-dimensional constraint and derive the form of the associated reactive stresses. To this end, we define for every point on the mid-surface a reference configuration that is mid-surface incompressible at that point. This family of reference configurations then allows us to determine the general form of the reactive stress tensor associated with the mid-surface incompressibility constraint. This derivation is most conveniently expressed using the Lagrangian parametrization so that we only use the Eulerian parametrization after establishing the general form of the reactive stresses.

We begin by introducing the notion of a Lagrangian parametrization, which we denote by $\{\xi_i\}_{i=1,2,3}$. In contrast to the Eulerian parametrization, the Lagrangian parametrization is time-independent [10, 11] but is otherwise analogous to the Eulerian parametrization (see Sec. 2 of the main text). In the following, we denote all quantities expressed in the Lagrangian parametrization by a *hat* symbol. The introduction of the Lagrangian parametrization is motivated by its use in the framework of constraint stresses in Ref. [12] and its convenient use for elastic material models.

To proceed, we assume there exists a *stress-free* reference configuration of the membrane with respect to which we define the mid-surface stretch. In addition, for every point $\boldsymbol{x}_0 \in \mathcal{S}_0$ on the mid-surface, we define a local reference configuration that is *mid-surface area incompressible* and denote quantities associated with it by a *dagger* symbol. More precisely, consider a point in parametric space, $(\bar{\xi}^1, \bar{\xi}^2)$, and its counterpart in physical space $\hat{\boldsymbol{x}}_0(\bar{\xi}^{\alpha}, t^*)$ at time $t^*$. The corresponding *mid-surface area incompressible* reference configuration then satisfies $\hat{J}^{\dagger}_0(\bar{\xi}^{\alpha}, t^*) = 1$ and the conditions

$$\hat{\boldsymbol{x}}^{\dagger}_0(\bar{\xi}^{\alpha}, t^*) = \hat{\boldsymbol{x}}_0(\bar{\xi}^{\alpha}, t^*) = \hat{\boldsymbol{x}}^*_0\ , \tag{75}$$

$$\hat{\boldsymbol{n}}^{\dagger}(\bar{\xi}^{\alpha}, t^*) = \hat{\boldsymbol{n}}(\bar{\xi}^{\alpha}, t^*)\ , \tag{76}$$

$$\hat{H}^{\dagger}(\bar{\xi}^{\alpha}, t^*) = \hat{H}(\bar{\xi}^{\alpha}, t^*)\ , \tag{77}$$

$$\hat{K}^{\dagger}(\bar{\xi}^{\alpha}, t^*) = \hat{K}(\bar{\xi}^{\alpha}, t^*)\ . \tag{78}$$

Equations (75)–(78) describe that the current and *mid-surface area incompressible* reference configurations are locally identical up to the surface stretch.

To formulate the mid-surface incompressibility constraint using the *mid-surface area incompressible* reference configuration, we express the deformation gradient $\hat{\boldsymbol{F}}^{\dagger} = \frac{\partial \hat{\boldsymbol{x}}}{\partial \hat{\boldsymbol{x}}^{\dagger}}$ using the basis

vectors $\hat{\boldsymbol{g}}_i^\dagger$ and $\hat{\boldsymbol{g}}_i$ of the mid-surface incompressible and current configurations as

$$\hat{\boldsymbol{F}}^\dagger = \hat{\boldsymbol{g}}_i \otimes \hat{\boldsymbol{g}}^{i\dagger} \ . \tag{79}$$

From Eq. (79), it follows that the right Cauchy-Green tensor associated with the mid-surface incompressible and current configurations can be written as

$$\hat{\boldsymbol{C}}^\dagger = \hat{\boldsymbol{F}}^{\dagger T} \hat{\boldsymbol{F}}^\dagger = \hat{g}_{ij}\, \hat{g}^{\dagger jk} \hat{\boldsymbol{g}}^{\dagger i} \otimes \hat{\boldsymbol{g}}_k^\dagger \ , \tag{80}$$

where $\hat{g}_{ij}$ and $\hat{g}^{\dagger ij}$ are the metric tensors of the current and mid-surface incompressible configurations, respectively. Using the determinant of the right Cauchy Green tensor under the assumption of Kirchhoff-Love kinematics [2,4–6], we can express the change of volume $\frac{\mathrm{d}\hat{v}}{\mathrm{d}\hat{v}^\dagger}$ between the mid-surface incompressible and current configurations as

$$\det \hat{\boldsymbol{C}}^\dagger = \frac{\mathrm{d}\hat{v}}{\mathrm{d}\hat{v}^\dagger} = \frac{\mathrm{d}\hat{a}_0 \left(1 - \delta \hat{H} \Theta + \frac{\delta^2}{4} \hat{K} \Theta^2\right)}{\mathrm{d}\hat{a}_0^\dagger \left(1 - \delta \hat{H}^\dagger \Theta + \frac{\delta^2}{4} \hat{K}^\dagger \Theta^2\right)} = \frac{\mathrm{d}\hat{a}_0}{\mathrm{d}\hat{a}_0^\dagger} \ , \tag{81}$$

where we used Eqs. (77) and (78), and defined $\mathrm{d}\hat{a}_0^\dagger$ and $\mathrm{d}\hat{a}_0$ as corresponding mid-surface area elements in the mid-surface incompressible and current configurations, respectively.

According to Eq. (81), we can express the mid-surface incompressibility constraint as

$$\hat{\Gamma}\left(\boldsymbol{C}^\dagger\right) = \det \hat{\boldsymbol{C}}^\dagger - 1 = 0 \ , \tag{82}$$

and following the procedure described in Ref. [12] yields the Cauchy stress[2],

$$\hat{\boldsymbol{\sigma}}_{\mathrm{r}} = \hat{\lambda} \frac{1}{\sqrt{\det \hat{\boldsymbol{C}}^\dagger}} \hat{\boldsymbol{F}}^\dagger \frac{\partial \Gamma}{\partial \hat{\boldsymbol{C}}^\dagger} \hat{\boldsymbol{F}}^{\dagger T} \ , \tag{83}$$

where $\hat{\lambda}$ is a factor that needs to be determined alongside all other unknowns. We can now use Jacobi's formula to find that the reactive stresses take the form

$$\hat{\boldsymbol{\sigma}}_{\mathrm{r}} = \hat{\hat{\lambda}} \boldsymbol{1} \ , \tag{84}$$

where all scalars have been lumped into the unknown $\hat{\hat{\lambda}}$. In part 2 [1], we described in detail that the stress components $\sigma_{i3} = \sigma_{3i}$ are determined by the reactive stresses required to enforce the Kirchhoff-Love assumptions. Therefore, it is sufficient to only consider the components of Eq. (84) along the in-plane directions, i.e.,

$$\hat{\boldsymbol{\sigma}}_{\mathrm{r}} = \hat{\hat{\lambda}} \boldsymbol{i} = \hat{\hat{\lambda}}\, \boldsymbol{a}_\alpha \otimes \boldsymbol{a}^\alpha \ . \tag{85}$$

Furthermore, by expressing Eq. (85) in the Eulerian parametrization, we can analogous write

$$\boldsymbol{\sigma}_{\mathrm{r}} = \tilde{\lambda} \boldsymbol{i} \ . \tag{86}$$

[2] In Eq. (83), the factor $1/\hat{J}^\dagger$ arising from the push-forward of the second Piola-Kirchhoff stress was lumped into the undetermined prefactor $\hat{\lambda}$.

To incorporate the reactive stresses in Eq. (86) into the $(2+\delta)$-dimensional theory, we express the stress vectors associated with $\boldsymbol{\sigma}_{\mathrm{r}}$ in terms of Chebyshev polynomials. To that end, we first write $\tilde{\lambda}$ using a generic series expansion as

$$\tilde{\lambda} = \sum_{k=0}^{\infty} \tilde{\lambda}_k \, \Theta^k \ . \tag{87}$$

Using the contravariant basis vector expansion in Eq. (1), the stress vector $\boldsymbol{T}_{\mathrm{r}}^{\alpha} = \boldsymbol{\sigma}_{\mathrm{r}}^T \boldsymbol{g}^{\alpha}$ becomes

$$\boldsymbol{T}_{\mathrm{r}}^{\alpha} = \sum_{m=0}^{\infty} \sum_{k=0}^{\infty} \frac{1}{2^m} \tilde{\lambda}_k \, \tilde{\boldsymbol{b}}^m \boldsymbol{a}^{\alpha} \, \Theta^{m+k} \tag{88}$$

$$= \sum_{m=0}^{\infty} \sum_{k=0}^{\infty} \frac{1}{2^m} \tilde{\lambda}_k \, \tilde{\boldsymbol{b}}^m \boldsymbol{a}^{\alpha} \sum_{l=0}^{m+k} c_l \alpha_{(m+k)l} P_l(\Theta) \ , \tag{89}$$

yielding the reactive stress contributions to $N^{\alpha\beta}$ and $M^{\alpha\beta}$,

$$N_{\mathrm{r}}^{\alpha\beta} = \frac{\delta}{2} \sum_{m=0}^{\infty} \sum_{k=0}^{\infty} \frac{1}{2^m} \tilde{\lambda}_k \, \boldsymbol{a}^{\beta} \cdot \tilde{\boldsymbol{b}}^m \boldsymbol{a}^{\alpha} \alpha_{(m+k)0} \ , \tag{90}$$

$$M_{\mathrm{r}}^{\alpha\beta} = -\frac{\delta^2}{4} \sum_{m=0}^{\infty} \sum_{k=0}^{\infty} \frac{1}{2^m} \tilde{\lambda}_k \, \boldsymbol{a}^{\beta} \cdot \tilde{\boldsymbol{b}}^m \boldsymbol{a}^{\alpha} \alpha_{(m+k)1} \ . \tag{91}$$

Since the reactive stresses enforce the mid-surface to be incompressible, we assume that only terms that are even about the mid-surface are non-zero i.e. $\lambda_{2i+1} = 0$, $i = 0, 1, 2 \ldots$ . By only keeping terms to the lowest non-vanishing order in the curvature tensor based on Eq. (21), Eqs. (90) and (91) then simplify to

$$N_{\mathrm{r}}^{\alpha\beta} = \left( \frac{\delta}{2} \sum_{m=0}^{\infty} \tilde{\lambda}_{2m} \alpha_{(2m)0} \right) a^{\alpha\beta} + \mathcal{O}\big(\tilde{\kappa}^2\big) \ , \tag{92}$$

$$M_{\mathrm{r}}^{\alpha\beta} = \left( -\frac{\delta^3}{8} \sum_{m=0}^{\infty} \tilde{\lambda}_{2m} \alpha_{(2m+1)1} \right) b^{\alpha\beta} + \mathcal{O}\big(\tilde{\kappa}^3\big) \ . \tag{93}$$

Finally, we also derive the contribution $\delta \boldsymbol{T}_{\mathrm{r}2}^{\alpha} = 2\langle \boldsymbol{T}_{\mathrm{r}}^{\alpha}, P_2(\Theta) \rangle$ required for the evaluation of the first-order boundary conditions. From Eq. (89), we immediately find

$$\delta \boldsymbol{T}_{2,\mathrm{r}}^{\alpha} = \delta \sum_{m=2}^{\infty} \sum_{l=0}^{m} \frac{1}{2^l} \tilde{\lambda}_{m-l} \, \tilde{\boldsymbol{b}}^l \boldsymbol{a}^{\alpha} \alpha_{m2} \ , \tag{94}$$

where the summation begins at $m = 2$ since $\alpha_{mk} = 0$ for $m < k$. Furthermore, note that we do not simplify Eq. (94) here as its contribution vanishes identically in the boundary conditions.

## 3 Equations of Motion

In Sec. 2, we obtained expressions for the elastic, viscous, and reactive stress contributions to $N^{\alpha\beta}$ and $M^{\alpha\beta}$. In this section, we derive the associated terms in the equations of motion, used in Sec. 5

of the main text. In particular, the in-plane equations require an expression for

$$N^{\gamma\alpha}_{;\gamma} + b^{\alpha}_{\gamma} M^{\lambda\gamma}_{;\lambda} + 2H_{,\gamma} M^{\gamma\alpha} \ , \tag{95}$$

while the shape equation requires an expression for

$$N^{\alpha\beta} b_{\alpha\beta} - M^{\beta\alpha}_{;\beta\alpha} \ . \tag{96}$$

### 3.1 Elastic Response

We begin by evaluating the elastic contributions to the terms of the in-plane equations in Eq. (95). Taking the covariant derivative of $N^{\alpha\beta}_{\mathrm{el}}$ in Eq. (26) and using Ricci's theorem,

$$a^{\alpha\beta}_{;\gamma} = 0 \ , \tag{97}$$

and the Mainardi-Codazzi relation

$$b^{\alpha}_{\beta;\gamma} = b^{\alpha}_{\gamma;\beta} \ , \tag{98}$$

leads to the expression

$$\begin{aligned}\left(N^{\beta\alpha}_{\mathrm{el}}\right)_{;\beta} = 2\bar{k}_{\mathrm{c}} J_{0,\beta} a^{\alpha\beta} + J_{0,\beta} k_{\mathrm{b}} \left(-\left(H - C\right)\left(2Ca^{\alpha\beta} + b^{\alpha\beta}\right) + \frac{1}{2}\left(K - G\right) a^{\alpha\beta}\right) \\ + J_0 k_{\mathrm{b}} \left[\left(-2C\left(H - C\right)_{,\beta} - 2\left(H - C\right)\left(H + C\right)_{,\beta} + \frac{1}{2}\left(K - G\right)_{,\beta}\right) a^{\alpha\beta} \right. \\ \left. - \left(H - C\right)_{,\beta} b^{\alpha\beta}\right] \ . \end{aligned} \tag{99}$$

Likewise, we take the covariant derivative of Eq. (34) and use Eqs. (97) and (98) to obtain

$$\left(M^{\gamma\beta}_{\mathrm{el}}\right)_{;\gamma} b^{\alpha}_{\beta} = -\frac{k_{\mathrm{b}}}{2} J_{0,\gamma} b^{\gamma\beta} b^{\alpha}_{\beta} - k_{\mathrm{b}} \left(J_0 - 1\right) H_{,\gamma} b^{\gamma\alpha} + k_{\mathrm{b}} \left(J_0 \left(H - C\right)\right)_{,\gamma} b^{\gamma\alpha} \ . \tag{100}$$

Furthermore, the last remaining term of Eq. (95) can be written as

$$2H_{,\gamma} M^{\gamma\alpha}_{\mathrm{el}} = -k_{\mathrm{b}} \left(J_0 - 1\right) H_{,\gamma} b^{\gamma\alpha} + 2J_0 k_{\mathrm{b}} \left(H - C\right) H_{,\gamma} a^{\gamma\alpha} \ . \tag{101}$$

Combining Eqs. (99)–(101) provides the elastic contribution to the in-plane equations as

$$\begin{aligned} & N^{\gamma\alpha}_{\mathrm{el};\gamma} + M^{\lambda\gamma}_{\mathrm{el};\lambda} b^{\alpha}_{\gamma} + 2H_{,\gamma} M^{\gamma\alpha}_{\mathrm{el}} \\ & \quad = J_{0,\beta} \left(2\bar{k}_{\mathrm{c}} a^{\alpha\beta} + k_{\mathrm{b}} \left(\boxed{-2\left(H - C\right) C a^{\alpha\beta} + \frac{1}{2}\left(K - G\right) a^{\alpha\beta}} - \boxed{\frac{1}{2} b^{\beta\gamma} b^{\alpha}_{\gamma}}\right)\right) \\ & \qquad - \boxed{2k_{\mathrm{b}} \left(J_0 - 1\right) H_{,\gamma} b^{\gamma\alpha}} + J_0 k_{\mathrm{b}} \left(-2\left(C\left(H - C\right)\right)_{,\beta} + \frac{1}{2}\left(K - G\right)_{,\beta}\right) a^{\alpha\beta} \ . \end{aligned} \tag{102}$$

From the relation between the bending rigidity and bulk modulus, $k_{\mathrm{b}} = \frac{\bar{k}_{\mathrm{c}}\delta^2}{2}$, and the assumption of small curvatures in the current and stress-free reference configurations (see Secs. 3 and 4.1 of the main text), it follows that the terms highlighted in blue in Eq. (102) are small and can be neglected.

Additionally invoking Eq. (21) shows the term highlighted in orange in Eq. (102) is negligible as well. By further employing Eq. (21) with $\boldsymbol{c} \equiv H_{,\gamma}\boldsymbol{a}^{\gamma}$ and the assumption that the length scale characterizing changes in curvature is not much smaller than the length scale characterizing changes in stresses (see Sec. 3 of the main text), we also find that the term highlighted in green in Eq. (102) can be neglected[3]. This simplifies the elastic contribution to the in-plane equations to

$$N^{\gamma\alpha}_{\mathrm{el};\gamma} + M^{\lambda\gamma}_{\mathrm{el};\lambda} b^{\alpha}_{\gamma} + 2H_{,\gamma} M^{\gamma\alpha}_{\mathrm{el}} \approx 2\bar{k}_{\mathrm{c}} J_{0,\beta} a^{\alpha\beta} + J_0 k_{\mathrm{b}} \left( -2 \left( C \left( H - C \right) \right)_{,\beta} + \frac{1}{2} \left( K - G \right)_{,\beta} \right) a^{\alpha\beta} \ . \tag{103}$$

Next, we turn our attention to the shape equation terms in Eq. (96). By contracting Eq. (26) with the curvature tensor, we find

$$N^{\alpha\beta}_{\mathrm{el}} b_{\alpha\beta} = 4\bar{k}_{\mathrm{c}} \left( J_0 - 1 \right) H - 2 J_0 k_{\mathrm{b}} \left( H - C \right) \left( 2H^2 + 2CH - K \right) + J_0 k_{\mathrm{b}} \left( K - G \right) H \ , \tag{104}$$

where we used the Cayley-Hamilton theorem to obtain

$$b^{\alpha\beta} b_{\alpha\beta} = 4H^2 - 2K \ . \tag{105}$$

Furthermore, we take covariant derivatives of Eq. (34) and use Ricci's theorem and the Mainardi-Codazzi relation in Eqs. (97) and (98) to find

$$\left( M^{\beta\alpha}_{\mathrm{el}} \right)_{;\beta\alpha} = -\frac{k_{\mathrm{b}}}{2} \left( J_{0,\beta} \right)_{:\alpha} b^{\alpha\beta} - 2 k_{\mathrm{b}} J_{0,\beta} H_{,\alpha} a^{\alpha\beta} - k_{\mathrm{b}} \left( J_0 - 1 \right) \Delta_{\mathrm{s}} H + k_{\mathrm{b}} \Delta_{\mathrm{s}} \left( J_0 \left( H - C \right) \right) \ , \tag{106}$$

with the definition of the surface Laplacian $\Delta_{\mathrm{s}}(\bullet) = \left( (\bullet)_{,\alpha} \right)_{:\beta} a^{\alpha\beta}$.

We can now write the elastic contribution to the shape equation as

$$\begin{aligned} N^{\alpha\beta}_{\mathrm{el}} b_{\alpha\beta} - \left( M^{\beta\alpha}_{\mathrm{el}} \right)_{;\beta\alpha} = {} & J_0 k_{\mathrm{b}} \left[ -2 \left( H - C \right) \left( 2H^2 + 2CH - K \right) + \left( K - G \right) H - \Delta_{\mathrm{s}} \left( H - C \right) \right] \\ & + k_{\mathrm{b}} \left( \frac{1}{2} J_{0,\alpha\beta} \, b^{\alpha\beta} + 2 J_{0,\beta} H_{,\alpha} a^{\alpha\beta} - J_{0,\alpha\beta} \, a^{\alpha\beta} \left( H - C \right) \right) \\ & + \left( J_0 - 1 \right) \left( 4\bar{k}_{\mathrm{c}} H + k_{\mathrm{b}} \Delta_{\mathrm{s}} H \right) \ . \end{aligned} \tag{107}$$

To simplify this expression further, recall that we assume the characteristic in-plane length scales for the curvature $\ell_{\mathrm{c}}$ and stresses $\ell_{\mathrm{s}}$ are large compared to the thickness (Sec. 3, main text). In particular, we assume $\ell_{\mathrm{s}}$ also characterizes changes in the mid-surface stretch $J_0$. We may then additionally invoke that for an arbitrary tensor $\boldsymbol{A} = A_{\alpha}^{\cdot\beta} \, \boldsymbol{a}^{\alpha} \otimes \boldsymbol{a}_{\beta}$,

$$\left( \delta \boldsymbol{b} \right)^m : \boldsymbol{A} = \mathcal{O}((\delta\kappa)^m) \left( \boldsymbol{i} : \boldsymbol{A} \right) \ , \tag{108}$$

allowung us to neglect the terms highlighted in green in Eq. (107). These simplifications result in

$$\begin{aligned} N^{\alpha\beta}_{\mathrm{el}} b_{\alpha\beta} - \left( M^{\beta\alpha}_{\mathrm{el}} \right)_{;\beta\alpha} \approx {} & J_0 k_{\mathrm{b}} \left[ -2 \left( H - C \right) \left( 2H^2 + 2CH - K \right) + \left( K - G \right) H \right] \\ & - J_0 k_{\mathrm{b}} \Delta_{\mathrm{s}} \left( H - C \right) + 4\bar{k}_{\mathrm{c}} \left( J_0 - 1 \right) H \ . \end{aligned} \tag{109}$$

[3] As a result of the stresses depending on the curvatures, the distinction between the characteristic length scale for the stresses $\ell_{\mathrm{s}}$ and curvatures $\ell_{\mathrm{c}}$ becomes obscure. To reconcile the notion of these length scales, $\ell_{\mathrm{s}}$ should be understood as the fastest varying length scale of any contribution to the stresses.

### 3.2 Viscous Response

We begin by evaluating the viscous contribution to the terms of the in-plane equations in Eq. (95). Recall, however, that we assume the viscous moments vanish, i.e. $M^{\alpha\beta}_{\mathrm{visc}} = 0$, implying that only the term $\pi^{\beta\alpha}_{;\beta}$ is required. Taking the covariant derivative of Eq. (62) and using Ricci's theorem and the Mainardi-Codazzi relation in Eqs. (97) and (98) then yields

$$\pi^{\beta\alpha}_{;\beta} = 2\zeta\left(d^{\beta\alpha}_{0;\beta} - v^3_{0,\beta}b^{\beta\alpha} - 2v^3_0 H_{,\beta}a^{\beta\alpha}\right) + \bar{\omega}\left(v^\alpha_{0:\alpha} - 2v^3_0 H\right)_{,\beta} a^{\alpha\beta} \ . \tag{110}$$

Similarly, invoking Eq. (105), $a^{\alpha\beta}b_{\alpha\beta} = 2H$, and $M^{\alpha\beta}_{\mathrm{visc}} = 0$ reduces the viscous contribution to the shape equation in Eq. (96) to

$$\pi^{\alpha\beta}b_{\alpha\beta} = 2\zeta\left(d^{\alpha\beta}_0 b_{\alpha\beta} - 2v^3_0\left(2H^2 - K\right)\right) + 2\bar{\omega}\left(v^\alpha_{0:\alpha} - 2v^3_0 H\right) H \ . \tag{111}$$

### 3.3 Reactive Stress Response

We now evaluate the contributions to Eqs. (95) and (96) arising from the reactive stresses associated with the mid-surface incompressibility constraint. By substituting Eqs. (92) and (93) into Eq. (95), we obtain

$$\begin{aligned} N^{\gamma\alpha}_{\mathrm{r};\gamma} + M^{\lambda\gamma}_{\mathrm{r};\lambda}b^\alpha_\gamma + 2H_{,\gamma}M^{\gamma\alpha}_{\mathrm{r}} = &\left(\frac{\delta}{2}\sum_{m=0}^{\infty}\tilde{\lambda}_{2m}\alpha_{(2m)0}\right)_{,\gamma} a^{\gamma\alpha} - \left(\frac{\delta^3}{8}\sum_{m=0}^{\infty}\tilde{\lambda}_{2m}\alpha_{(2m+1)1}\right)_{,\lambda} b^{\lambda\gamma}b^\alpha_\gamma \\ &- 4\left(\frac{\delta^3}{8}\sum_{m=0}^{\infty}\tilde{\lambda}_{2m}\alpha_{(2m+1)1}\right) H_{,\gamma}b^{\gamma\alpha} \ , \end{aligned} \tag{112}$$

where we again applied Eqs. (97) and (98). By invoking the assumption $\ell_{\mathrm{c}}/\ell_{\mathrm{s}} \lll 1$ (Sec. 3, main text), with changes in $\tilde{\lambda}_m$ characterized by $\ell_{\mathrm{s}}$, Eq. (112) simplifies to

$$N^{\gamma\alpha}_{\mathrm{r};\gamma} + M^{\lambda\gamma}_{\mathrm{r};\lambda}b^\alpha_\gamma + 2H_{,\gamma}M^{\gamma\alpha}_{\mathrm{r}} \approx \left(\frac{\delta}{2}\sum_{m=0}^{\infty}\tilde{\lambda}_{2m}\alpha_{(2m)0}\right)_{,\gamma} a^{\gamma\alpha} \ . \tag{113}$$

Next, the reactive stress contribution to the shape equation is obtained as

$$N^{\alpha\beta}_{\mathrm{el}}b_{\alpha\beta} - \left(M^{\beta\alpha}_{\mathrm{el}}\right)_{;\beta\alpha} = 2\left(\frac{\delta}{2}\sum_{m=0}^{\infty}\tilde{\lambda}_{2m}\alpha_{(2m)0}\right) H + \left[\left(\frac{\delta^3}{8}\sum_{m=0}^{\infty}\tilde{\lambda}_{2m}\alpha_{(2m+1)1}\right) b^{\alpha\beta}\right]_{;\alpha\beta} \ , \tag{114}$$

which, upon using the assumptions of large in-plane length scales, becomes

$$N^{\alpha\beta}_{\mathrm{el}}b_{\alpha\beta} - \left(M^{\beta\alpha}_{\mathrm{el}}\right)_{;\beta\alpha} \approx 2\left(\frac{\delta}{2}\sum_{m=0}^{\infty}\tilde{\lambda}_{2m}\alpha_{(2m)0}\right) H \ . \tag{115}$$

Equations (113) and (115) suggest the definition of the effective surface tension $\lambda$ as

$$\lambda = \left(\frac{\delta}{2}\sum_{m=0}^{\infty}\tilde{\lambda}_{2m}\alpha_{(2m)0}\right) \ . \tag{116}$$

This definition simplifies Eqs. (113) and (115) to

$$N^{\gamma\alpha}_{\mathrm{r};\gamma} + M^{\lambda\gamma}_{\mathrm{r};\lambda} b^{\alpha}_{\gamma} + 2H_{,\gamma} M^{\gamma\alpha}_{\mathrm{r}} = \lambda_{,\gamma} a^{\gamma\alpha} \ , \tag{117}$$

$$N^{\alpha\beta}_{\mathrm{el}} b_{\alpha\beta} - \left(M^{\beta\alpha}_{\mathrm{el}}\right)_{;\beta\alpha} = 2\lambda H \ . \tag{118}$$

## 4 Traction Boundary Conditions

In this section, we use the expressions obtained for $N^{\alpha\beta}$, $M^{\alpha\beta}$, and $\boldsymbol{T}^{\alpha}_{2}$ in Sec. 2 to derive the in-plane traction boundary conditions (see Sec. 3 of the main text)

$$\check{\nu}_{\alpha}\left(N^{\alpha\beta} + b^{\alpha}_{\gamma} M^{\gamma\beta}\right) = \delta\langle \boldsymbol{a}^{\beta} \cdot \tilde{\bar{\boldsymbol{t}}}, P_0(\Theta)\rangle \ , \tag{119}$$

$$\check{\nu}_{\alpha}\left(M^{\alpha\beta} + \frac{\delta^2}{16} b^{\alpha}_{\gamma}\left(2N^{\gamma\beta} + \delta \boldsymbol{T}^{\alpha}_{2} \cdot \boldsymbol{a}^{\beta}\right)\right) = -\frac{\delta^2}{2}\langle \boldsymbol{a}^{\beta} \cdot \tilde{\bar{\boldsymbol{t}}}, P_1(\Theta)\rangle \ , \tag{120}$$

where $\boldsymbol{\nu} = \check{\nu}^{\alpha}\boldsymbol{a}_{\alpha}$ is the outward-pointing binormal vector of the mid-surface boundary.

**Elastic Response** To determine the elastic contribution to the zeroth-order boundary condition in Eq. (119), we substitute Eqs. (26) and (34) to find

$$\begin{aligned}\check{\nu}_{\alpha}\left(N^{\alpha\beta}_{\mathrm{el}} + b^{\alpha}_{\gamma} M^{\gamma\beta}_{\mathrm{el}}\right) &= \check{\nu}_{\alpha}\Bigg[(J_0 - 1)\left(2\bar{k}_{\mathrm{c}} a^{\alpha\beta} - \frac{k_{\mathrm{b}}}{2} b^{\alpha}_{\gamma} b^{\gamma\beta}\right) \\ &\qquad + J_0 k_{\mathrm{b}}\left(-2C a^{\alpha\beta}\left(H - C\right) + \frac{1}{2}\left(K - G\right) a^{\alpha\beta}\right)\Bigg] \qquad (121) \\ &\approx \check{\nu}^{\beta}\left(2\bar{k}_{\mathrm{c}}\left(J_0 - 1\right) + J_0 k_{\mathrm{b}}\left(-2C\left(H - C\right) + \frac{1}{2}\left(K - G\right)\right)\right) \ , \qquad (122)\end{aligned}$$

where we neglected the term highlighted in green based on Eq. (21). Similarly, we substitute Eqs. (26), (34), and (41) into the first-order boundary condition in Eq. (120) to obtain

$$\begin{aligned}&\check{\nu}_{\alpha}\left(M^{\alpha\beta}_{\mathrm{el}} + \frac{\delta^2}{16} b^{\alpha}_{\gamma}\left(2N^{\gamma\beta}_{\mathrm{el}} + \delta \boldsymbol{T}^{\alpha}_{2,\mathrm{el}} \cdot \boldsymbol{a}^{\beta}\right)\right) \\ &= \check{\nu}_{\alpha}\Bigg\{-\frac{k_{\mathrm{b}}}{2}\left(J_0 - 1\right) b^{\alpha\beta} + J_0 k_{\mathrm{b}}\left(H - C\right) a^{\alpha\beta} \\ &\quad + \frac{\delta^2}{16} b^{\alpha}_{\gamma}\Bigg[4\bar{k}_{\mathrm{c}}\left(J_0 - 1\right) a^{\alpha\beta} + 2J_0 k_{\mathrm{b}}\left(-\left(H - C\right)\left(2C a^{\alpha\beta} + b^{\alpha\beta}\right) + \frac{1}{2}\left(K - G\right) a^{\alpha\beta}\right) \\ &\quad + \frac{k_{\mathrm{b}}}{2}\left(J_0 - 1\right) b^{\alpha}_{\gamma} b^{\gamma\beta} + J_0 k_{\mathrm{b}}\left(-\left(H - C\right)\left(2C a^{\alpha\beta} + b^{\alpha\beta}\right) + \frac{1}{2}\left(K - G\right) a^{\alpha\beta}\right)\Bigg]\Bigg\} \ . \qquad (123)\end{aligned}$$

The terms highlighted in green in Eq. (123) can be neglected based on Eq. (21) and the assumption of small curvatures. This reduces Eq. (123) to

$$\begin{aligned}\check{\nu}_{\alpha}\left(M^{\alpha\beta}_{\mathrm{el}} + \frac{\delta^2}{16} b^{\alpha}_{\gamma}\left(2N^{\gamma\beta}_{\mathrm{el}} + \delta \boldsymbol{T}^{\alpha}_{2,\mathrm{el}} \cdot \boldsymbol{a}^{\beta}\right)\right) &\approx \check{\nu}_{\alpha}\Bigg(J_0 k_{\mathrm{b}}\left(H - C\right) a^{\alpha\beta} \\ &\qquad + \left(J_0 - 1\right) b^{\alpha\beta}\left(\frac{\delta^2 \bar{k}_{\mathrm{c}}}{4} - \frac{k_{\mathrm{b}}}{2}\right)\Bigg) \ . \qquad (124)\end{aligned}$$

**Viscous Response** Since we assume the viscous moments vanish, i.e. $M^{\alpha\beta}_{\text{visc}} = 0$, the viscous contribution to the zeroth-order boundary condition in Eq. (119) simpifies to

$$\check{\nu}_\alpha \left( \pi^{\alpha\beta} + b^\alpha_\gamma M^{\gamma\beta}_{\text{visc}} \right) = \check{\nu}_\alpha \pi^{\alpha\beta} \ , \tag{125}$$

with $\pi^{\alpha\beta}$ given by Eq. (62). Furthermore, comparison of $\boldsymbol{T}^\alpha_{2,\text{visc}} \cdot \boldsymbol{a}^\beta$ in Eq. (74) to $\pi^{\alpha\beta}$ in Eq. (62) shows that $\boldsymbol{T}^\alpha_{2,\text{visc}} \cdot \boldsymbol{a}^\beta$ can be neglected in the first-order boundary condition in Eq. (120). With $M^{\alpha\beta}_{\text{visc}} = 0$, this leads to

$$\check{\nu}_\alpha \left( M^{\alpha\beta}_{\text{visc}} + \frac{\delta^2}{16} b^\alpha_\gamma \left( 2\pi^{\gamma\beta} + \delta \boldsymbol{T}^\alpha_{2,\text{visc}} \cdot \boldsymbol{a}^\beta \right) \right) \approx \check{\nu}_\alpha \frac{\delta^2}{8} b^\alpha_\gamma \pi^{\gamma\beta} \ . \tag{126}$$

**Reactive Stress Response** To obtain the reactive stress contribution to Eq. (119), we substitute Eqs. (92) and (93) to obtain

$$\check{\nu}_\alpha \left( N^{\alpha\beta}_{\text{r}} + b^\alpha_\gamma M^{\gamma\beta}_{\text{r}} \right) = \check{\nu}_\alpha \left( \frac{\delta}{2} \sum_{m=0}^{\infty} \tilde{\lambda}_{2m} \alpha_{(2m)0} a^{\alpha\beta} - \frac{\delta^3}{8} b^\alpha_\gamma b^{\gamma\beta} \sum_{m=0}^{\infty} \tilde{\lambda}_{2m} \alpha_{(2m+1)1} \right) \tag{127}$$

$$\approx \check{\nu}^\beta \frac{\delta}{2} \sum_{m=0}^{\infty} \tilde{\lambda}_{2m} \alpha_{(2m)0} \tag{128}$$

$$= \check{\nu}^\beta \lambda \ , \tag{129}$$

where we neglected the term highlighted in green based on Eq. (21) and used the definition of the effective surface tension in Eq. (116). In contrast, the reactive stress contribution to the boundary condition in Eq. (120) vanishes identically. To show this, we insert the expressions for the reactive stresses, moments, and $\boldsymbol{T}^\alpha_{2,\text{r}}$ in Eqs. (90), (91), and (94), respectively, into Eq. (120) to find

$$\begin{aligned} &\check{\nu}_\alpha \left( M^{\alpha\beta}_{\text{r}} + \frac{\delta^2}{16} b^\alpha_\gamma \left( 2N^{\gamma\beta}_{\text{r}} + \delta \boldsymbol{T}^\alpha_{2,\text{r}} \cdot \boldsymbol{a}^\beta \right) \right) \\ &\quad = \check{\nu}_\alpha \Bigg\{ -\frac{\delta^2}{4} \sum_{m=0}^{\infty} \sum_{l=0}^{m} \frac{1}{2^l} \tilde{\lambda}_{m-l} \left[ \tilde{\boldsymbol{b}}^l \right]^{\alpha\beta} \alpha_{m1} \\ &\qquad + \frac{\delta^2}{16} \tilde{b}^\alpha_\gamma \left( \sum_{m=0}^{\infty} \sum_{l=0}^{m} \frac{1}{2^l} \tilde{\lambda}_{m-l} \left[ \tilde{\boldsymbol{b}}^l \right]^{\gamma\beta} \alpha_{m0} + \sum_{m=2}^{\infty} \sum_{l=0}^{m} \frac{1}{2^l} \tilde{\lambda}_{m-l} \left[ \tilde{\boldsymbol{b}}^l \right]^{\gamma\beta} \alpha_{m2} \right) \Bigg\} \ . \end{aligned} \tag{130}$$

To show that the right-hand side of Eq. (130) vanishes identically, we consider a fixed coefficient $\tilde{\lambda}_k$ with $k = m - l$. We then find that $\tilde{\lambda}_k$ in Eq. (130) gets multiplied by the factor

$$-\sum_{m=k}^{\infty} \frac{1}{2^{m-k}} \left[ \tilde{\boldsymbol{b}}^{m-k} \right]^{\alpha\beta} \alpha_{m1} + \frac{1}{4} \tilde{b}^\alpha_\gamma \left( \sum_{m=k}^{\infty} \frac{1}{2^{m-k}} \left[ \tilde{\boldsymbol{b}}^{m-k} \right]^{\gamma\beta} \alpha_{m0} + \sum_{m=k}^{\infty} \frac{1}{2^{m-k}} \left[ \tilde{\boldsymbol{b}}^{m-k} \right]^{\gamma\beta} \alpha_{m2} \right) \ . \tag{131}$$

To see that this factor vanishes, we can group terms of equal power in the curvature tensor, say $\left[\tilde{\boldsymbol{b}}^n\right]^{\gamma\beta}$ for $n \geq 1$. Then, we find that $\left[\tilde{\boldsymbol{b}}^n\right]^{\gamma\beta}$ gets multiplied by the term,

$$-\frac{1}{2^n}\alpha_{(n+k)1} + \frac{1}{2^{n+1}}\left(\alpha_{(n+k-1)0} + \alpha_{(n+k-1)2}\right) =$$
$$2^{1-2n-k}\left(-\binom{n+k}{\frac{n+k-1}{2}} + \binom{n+k-1}{\frac{n+k-1}{2}} + \binom{n+k-1}{\frac{n+k-1}{2}-1}\right) = 0 \ . \tag{132}$$

For $n = 0$, only the first sum of the right-hand side of Eq. (130) is non-vanishing, yielding the contribution

$$-\frac{\delta^2}{4}\sum_{m=0}^{\infty}\tilde{\lambda}_m\alpha_{m1}\, a^{\alpha\beta} = -\frac{\delta^2}{4}\sum_{m=0}^{\infty}\tilde{\lambda}_{2m+1}\alpha_{(2m+1)1}\, a^{\alpha\beta} = 0 \ , \tag{133}$$

where the first equality follows from Eq. (7) and the second equality is a result of the assumption that odd terms $\tilde{\lambda}_{2m+1}$ vanish. Therefore, Eq. (130) simplifies to

$$\check{\nu}_\alpha\left(M_{\mathrm{r}}^{\alpha\beta} + \frac{\delta^2}{16}b_\gamma^\alpha\left(2N_{\mathrm{r}}^{\gamma\beta} + \delta\boldsymbol{T}_{2,\mathrm{r}}^\alpha\cdot\boldsymbol{a}^\beta\right)\right) = 0 \ . \tag{134}$$

**Compressible in-plane traction boundary condition** Finally, we can combine Eqs. (122) and (125) to obtain the zeroth-order, in-plane traction boundary condition for the compressible case as

$$\check{\nu}^\beta\left(2\bar{k}_{\mathrm{c}}\left(J_0-1\right) + J_0 k_{\mathrm{b}}\left(-2C\left(H-C\right) + \frac{1}{2}\left(K-G\right)\right)\right) + \check{\nu}_\alpha\pi^{\alpha\beta} = \delta\langle\boldsymbol{a}^\beta\cdot\bar{\tilde{\boldsymbol{t}}}, P_0(\Theta)\rangle \ . \tag{135}$$

Similarly, we obtain the first-order, in-plane traction boundary condition from Eqs. (124) and (126) as

$$\check{\nu}_\alpha\left(J_0 k_{\mathrm{b}}\left(H-C\right)a^{\alpha\beta} + \left(J_0-1\right)b^{\alpha\beta}\left(\frac{\delta^2\bar{k}_{\mathrm{c}}}{4} - \frac{k_{\mathrm{b}}}{2}\right) + \frac{\delta^2}{8}b_\gamma^\alpha\pi^{\gamma\beta}\right) = -\frac{\delta^2}{4}\langle\boldsymbol{a}^\beta\cdot\bar{\tilde{\boldsymbol{t}}}, P_1(\Theta)\rangle \ . \tag{136}$$

By recalling the definition of the bending rigidity in terms of the membrane bulk modulus, $k_{\mathrm{b}} = \frac{\bar{k}_{\mathrm{c}}\delta^2}{2}$, we find that the term highlighted in green is identically zero, reducing Eq. (136) to

$$\check{\nu}_\alpha\left(J_0 k_{\mathrm{b}}\left(H-C\right)a^{\alpha\beta} + \frac{\delta^2}{8}b_\gamma^\alpha\pi^{\gamma\beta}\right) = -\frac{\delta^2}{4}\langle\boldsymbol{a}^\beta\cdot\bar{\tilde{\boldsymbol{t}}}, P_1(\Theta)\rangle \ . \tag{137}$$

**Incompressible in-plane traction boundary condition** The boundary conditions for the incompressible case are obtained from Eqs. (135) and (137) by additionally accounting for Eqs. (129) and (134) and setting $J_0 = 1$, yielding

$$\check{\nu}^\beta\left(\lambda + k_{\mathrm{b}}\left(-2C\left(H-C\right) + \frac{1}{2}\left(K-G\right)\right)\right) + \check{\nu}_\alpha\pi^{\alpha\beta} = \delta\langle\boldsymbol{a}^\beta\cdot\bar{\tilde{\boldsymbol{t}}}, P_0(\Theta)\rangle \ , \tag{138}$$

$$\check{\nu}_\alpha\left(k_{\mathrm{b}}\left(H-C\right)a^{\alpha\beta} + \frac{\delta^2}{8}b_\gamma^\alpha\pi^{\gamma\beta}\right) = -\frac{\delta^2}{2}\langle\boldsymbol{a}^\beta\cdot\bar{\tilde{\boldsymbol{t}}}, P_1(\Theta)\rangle \ . \tag{139}$$

# 5 Traction Boundary Conditions in Strict Surface Theories

The in-plane traction boundary conditions of strict surface theories are commonly given along the directions of the outward-pointing normal and tangent vectors to $\partial\mathcal{S}_0$ [10, 13]. In the following, we rewrite the in-plane boundary tractions $\boldsymbol{f}_{\mathrm{ip}}$ of strict surface theories along the parametric direction as done in the main text for the $(2+\delta)$-dimensional theory.

We begin by recalling that $\boldsymbol{\nu}$ denotes the outward-pointing normal on $\partial\mathcal{S}_0$ and that the tangent vector to $\partial\mathcal{S}_0$, $\boldsymbol{\tau}$, is given by

$$\boldsymbol{\tau} = \boldsymbol{n} \times \boldsymbol{\nu} \ . \tag{140}$$

With the traction components $f_\nu$ and $f_\tau$ along $\boldsymbol{\nu}$ and $\boldsymbol{\tau}$, respectively, we can write the in-plane boundary traction as

$$\boldsymbol{f}_{\mathrm{ip}} = f_\nu \boldsymbol{\nu} + f_\tau \boldsymbol{\tau} \ , \tag{141}$$

with the components $f_\nu$ and $f_\tau$ given by [13]

$$f_\nu = k_{\mathrm{b}} \Big[ (H-C)^2 - (H-C)\,\kappa_\nu \Big] - k_{\mathrm{g}}\xi^2 + 2k_{\mathrm{c}}\,(J_0 - 1) + \pi^{\alpha\beta}\check{\nu}_\alpha\check{\nu}_\beta \ , \tag{142}$$

$$f_\tau = -\xi \left[ k_{\mathrm{b}}\,(H-C) + k_{\mathrm{g}}\kappa_\tau \right] + \pi^{\alpha\beta}\tau_\alpha\check{\nu}_\beta \ . \tag{143}$$

Here, $\kappa_\nu$ and $\kappa_\tau$ are the curvatures along $\boldsymbol{\nu}$ and $\boldsymbol{\tau}$, respectively, and $\xi$ is the twist, given by

$$\kappa_\nu = \boldsymbol{\nu} \cdot \boldsymbol{b}\boldsymbol{\nu} \ , \tag{144}$$

$$\kappa_\tau = \boldsymbol{\tau} \cdot \boldsymbol{b}\boldsymbol{\tau} \ , \tag{145}$$

$$\xi = \boldsymbol{\nu} \cdot \boldsymbol{b}\boldsymbol{\tau} \ , \tag{146}$$

where $\boldsymbol{b}$ is the curvature tensor on the mid-surface.

For simplicity, we now consider the terms associated with $k_{\mathrm{b}}$, $k_{\mathrm{g}}$ and $\pi^{\alpha\beta}$ individually. By substituting Eqs. (142)–(146) into Eq. (141) and only considering the terms associated with the bending rigidity $k_{\mathrm{b}}$, we obtain

$$\boldsymbol{f}_{\mathrm{ip,b}} = k_{\mathrm{b}} \Big[ (H-C)^2\,\boldsymbol{\nu} - (H-C)\left( (\boldsymbol{\nu}\cdot\boldsymbol{b}\boldsymbol{\nu})\,\boldsymbol{\nu} + (\boldsymbol{\nu}\cdot\boldsymbol{b}\boldsymbol{\tau})\,\boldsymbol{\tau} \right) \Big] \tag{147}$$

$$= k_{\mathrm{b}} \Big[ (H-C)^2\,\boldsymbol{\nu} - (H-C)\,\boldsymbol{\nu}\cdot\boldsymbol{b}\,(\boldsymbol{\nu}\otimes\boldsymbol{\nu} + \boldsymbol{\tau}\otimes\boldsymbol{\tau}) \Big] \tag{148}$$

$$= k_{\mathrm{b}} \Big[ (H-C)^2\,\boldsymbol{\nu} - (H-C)\,\boldsymbol{\nu}\cdot\boldsymbol{b} \Big] \ , \tag{149}$$

where we have used $\boldsymbol{i} = \boldsymbol{\nu}\otimes\boldsymbol{\nu} + \boldsymbol{\tau}\otimes\boldsymbol{\tau}$ and $\boldsymbol{b}\boldsymbol{i} = \boldsymbol{b}$. Similarly, for the terms associated with the Gaussian bending rigidity $k_{\mathrm{g}}$, we find

$$\boldsymbol{f}_{\mathrm{ip,g}} = -k_{\mathrm{g}}\xi\,(\xi\boldsymbol{\nu} + \kappa_\tau\boldsymbol{\tau}) \tag{150}$$

$$= -k_{\mathrm{g}}\boldsymbol{\nu}\cdot\boldsymbol{b}\boldsymbol{\tau}\,\left( (\boldsymbol{\nu}\cdot\boldsymbol{b}\boldsymbol{\tau})\,\boldsymbol{\nu} + (\boldsymbol{\tau}\cdot\boldsymbol{b}\boldsymbol{\tau})\,\boldsymbol{\tau} \right) \ . \tag{151}$$

Using the symmetry of the curvature tensor then yields

$$\boldsymbol{f}_{\mathrm{ip,g}} = -k_{\mathrm{g}}\,(\boldsymbol{\nu}\cdot\boldsymbol{b}\boldsymbol{\tau})\,\boldsymbol{\tau}\cdot\boldsymbol{b}\,(\boldsymbol{\nu}\otimes\boldsymbol{\nu} + \boldsymbol{\tau}\otimes\boldsymbol{\tau}) \tag{152}$$

$$= -k_{\mathrm{g}}\,(\boldsymbol{\nu}\cdot\boldsymbol{b}\boldsymbol{\tau})\,\boldsymbol{\tau}\cdot\boldsymbol{b} \ . \tag{153}$$

Finally, with $\boldsymbol{\pi} = \pi^{\alpha\beta} \boldsymbol{a}_\alpha \otimes \boldsymbol{a}_\beta$, we write the viscous contribution to Eq. (141) as

$$\begin{aligned} \boldsymbol{f}_{\mathrm{ip,v}} &= (\boldsymbol{\nu} \cdot \boldsymbol{\pi}\boldsymbol{\nu})\, \boldsymbol{\nu} + (\boldsymbol{\tau} \cdot \boldsymbol{\pi}\boldsymbol{\nu})\, \boldsymbol{\tau} && (154) \\ &= \boldsymbol{\nu} \cdot \boldsymbol{\pi}\, (\boldsymbol{\nu} \otimes \boldsymbol{\nu} + \boldsymbol{\tau} \otimes \boldsymbol{\tau}) && (155) \\ &= \boldsymbol{\nu} \cdot \boldsymbol{\pi}\ , && (156) \end{aligned}$$

where we now also used the symmetry of $\boldsymbol{\pi}$. Finally, taking the dot product of Eq. (141) with $\boldsymbol{a}^\alpha$ and substituting Eqs. (149), (153) and (156) yields the in-plane boundary traction along $\boldsymbol{a}^\alpha$ as

$$f^\alpha_{\mathrm{ip}} = k_{\mathrm{b}} \Big[ (H - C)^2\, \check{\nu}^\alpha - (H - C)\, \check{\nu}_\beta b^{\beta\alpha} \Big] - k_{\mathrm{g}} \check{\nu}_\beta b^{\beta\gamma} \tau_\gamma \tau_\mu b^{\mu\alpha} + 2k_{\mathrm{c}}\, (J_0 - 1)\, \check{\nu}^\alpha + \check{\nu}_\beta \pi^{\beta\alpha}\ . \qquad (157)$$

# References


[1] Omar, Y. A., Lipel, Z. G. & Mandadapu, K. K. The $(2+\delta)$-dimensional theory of the electromechanics of lipid membranes: II. Balance laws. *arXiv preprint arXiv:2309.03863* (2023).

[2] Song, Z. & Dai, H.-H. On a consistent finite-strain shell theory based on 3-d nonlinear elasticity. *International Journal of Solids and Structures* **97**, 137–149 (2016).

[3] Cody, W. A survey of practical rational and polynomial approximation of functions. *SIAM Review* **12**, 400–423 (1970).

[4] Chien, W.-Z. The intrinsic theory of thin shells and plates: I. General theory. *Quarterly of Applied Mathematics* **1**, 297–327 (1944).

[5] Green, A. & Zerna, W. The equilibrium of thin elastic shells. *The Quarterly Journal of Mechanics and Applied Mathematics* **3**, 9–22 (1950).

[6] Naghdi, P. M. Foundations of elastic shell theory. Tech. Rep., Institute of Engineering Research, University of California, Berkeley (1962).

[7] Evans, E. A., Waugh, R. & Melnik, L. Elastic area compressibility modulus of red cell membrane. *Biophysical Journal* **16**, 585–595 (1976).

[8] Nichol, J. & Hutter, O. Tensile strength and dilatational elasticity of giant sarcolemmal vesicles shed from rabbit muscle. *The Journal of Physiology* **493**, 187–198 (1996).

[9] Evans, E. A. *Mechanics and thermodynamics of biomembranes* (CRC press, 2018).

[10] Rangamani, P., Agrawal, A., Mandadapu, K. K., Oster, G. & Steigmann, D. J. Interaction between surface shape and intra-surface viscous flow on lipid membranes. *Biomechanics and Modeling in Mechanobiology* **12**, 833–845 (2013).

[11] Sahu, A., Omar, Y. A., Sauer, R. A. & Mandadapu, K. K. Arbitrary lagrangian–eulerian finite element method for curved and deforming surfaces: I. General theory and application to fluid interfaces. *Journal of Computational Physics* **407**, 109253 (2020).

[12] Carlson, D. E., Fried, E. & Tortorelli, D. A. Geometrically-based consequences of internal constraints. In *The Rational Spirit in Modern Continuum Mechanics*, 141–149 (Springer, 2004).

[13] Sahu, A., Sauer, R. A. & Mandadapu, K. K. Irreversible thermodynamics of curved lipid membranes. *Physical Review E* **96**, 042409 (2017).
